# Supplementary material for: Exploring specialization and sensitivity of convolutional neural networks under simultaneous image augmentations
Source: arXiv:2503.03283 ancillary file (2026-11-07)
Supplement: Supplementary file 1 [file SupplementaryS7.pdf]

# Exploring specialization and sensitivity of convolutional neural networks in the context of simultaneous image augmentations – supplementary material (S7)

Pavel Kharyuk, Sergey Matveev, Ivan Oseledets

## Contents

**1 Variances and coefficients of variation (CVs) 2**
1.1 AlexNet . . . . . 2
1.2 VGG11 . . . . . 6
1.3 ResNet18 . . . . . 10

**2 Correlation between pairs of augmentation variables within selected sensitivity values 14**

**3 Spatial maps for unit-wise correlations between sensitivities and coefficients of variation 18**

**4 Confusion matrices from Linear Discriminant Analysis (LDA) of the estimated sensitivities 21**

**5 Masked activations: hierarchical clustering analysis (HCA) of the prediction patterns 23**

**6 Single-class sensitivity analysis: relating single-class sensitivities and masked-activation predictions 27**

**7 Correlation matrices between sensitivity variables 30**

# 1 Variances and coefficients of variation (CVs)

## 1.1 AlexNet

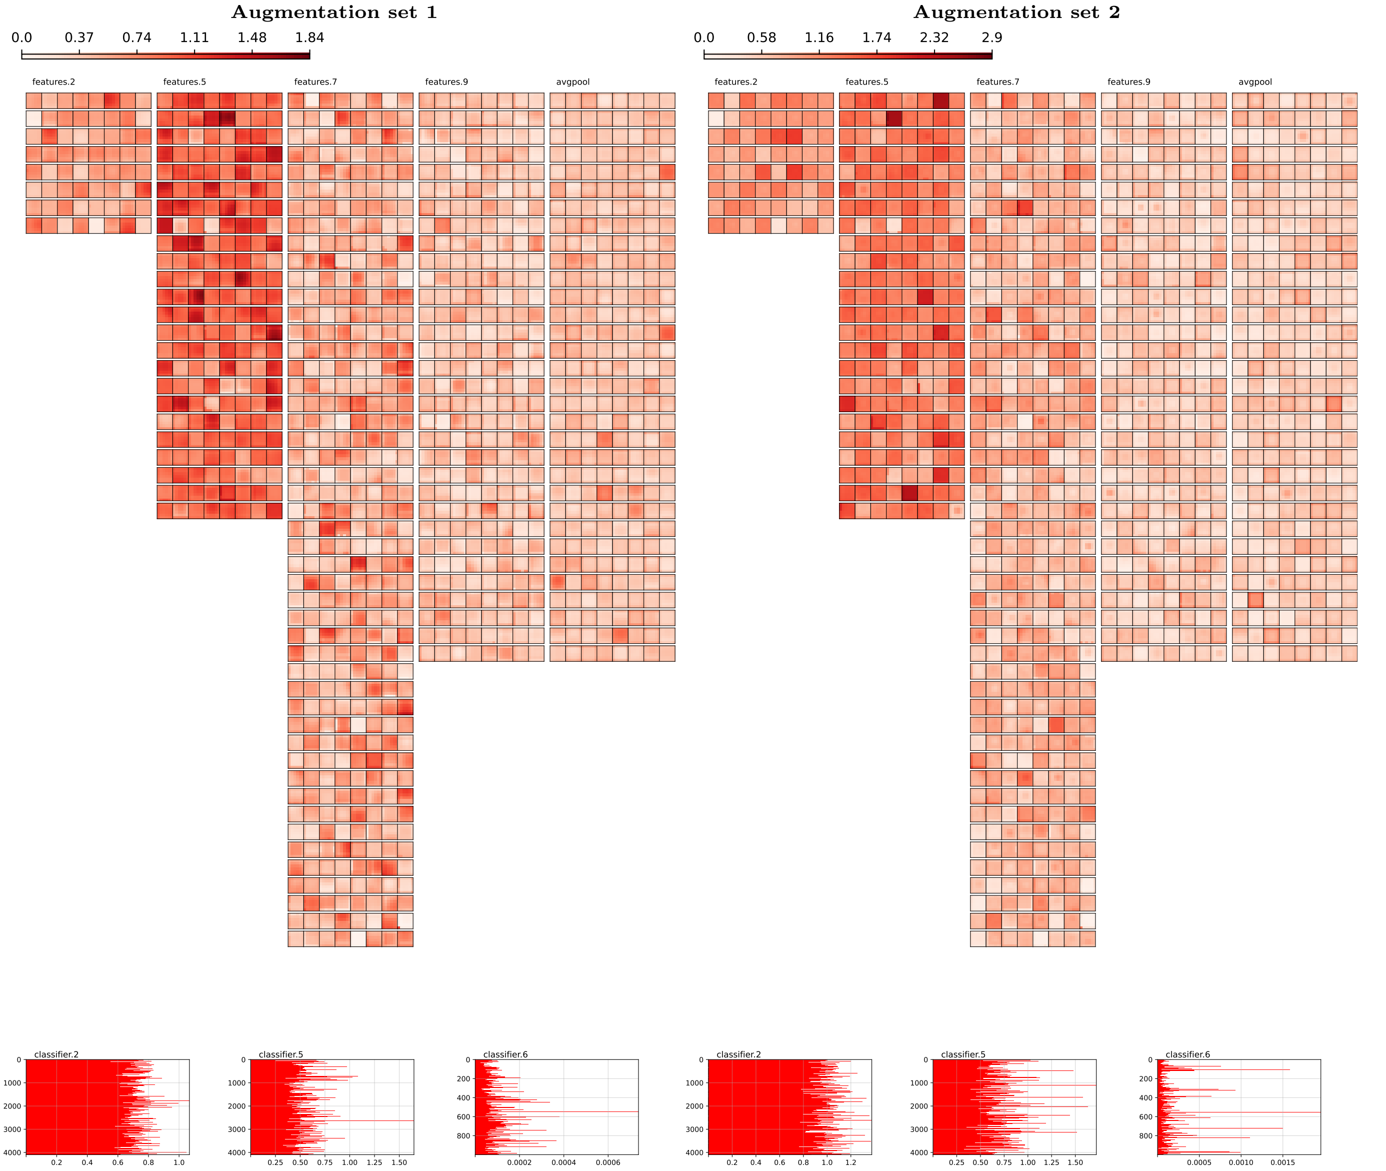


Figure S7.1.1 (a): Variances of activations plotted on a log scale ($\log_{10}(1+v)$). AlexNet network, Sobol indices (sampling scheme 1).

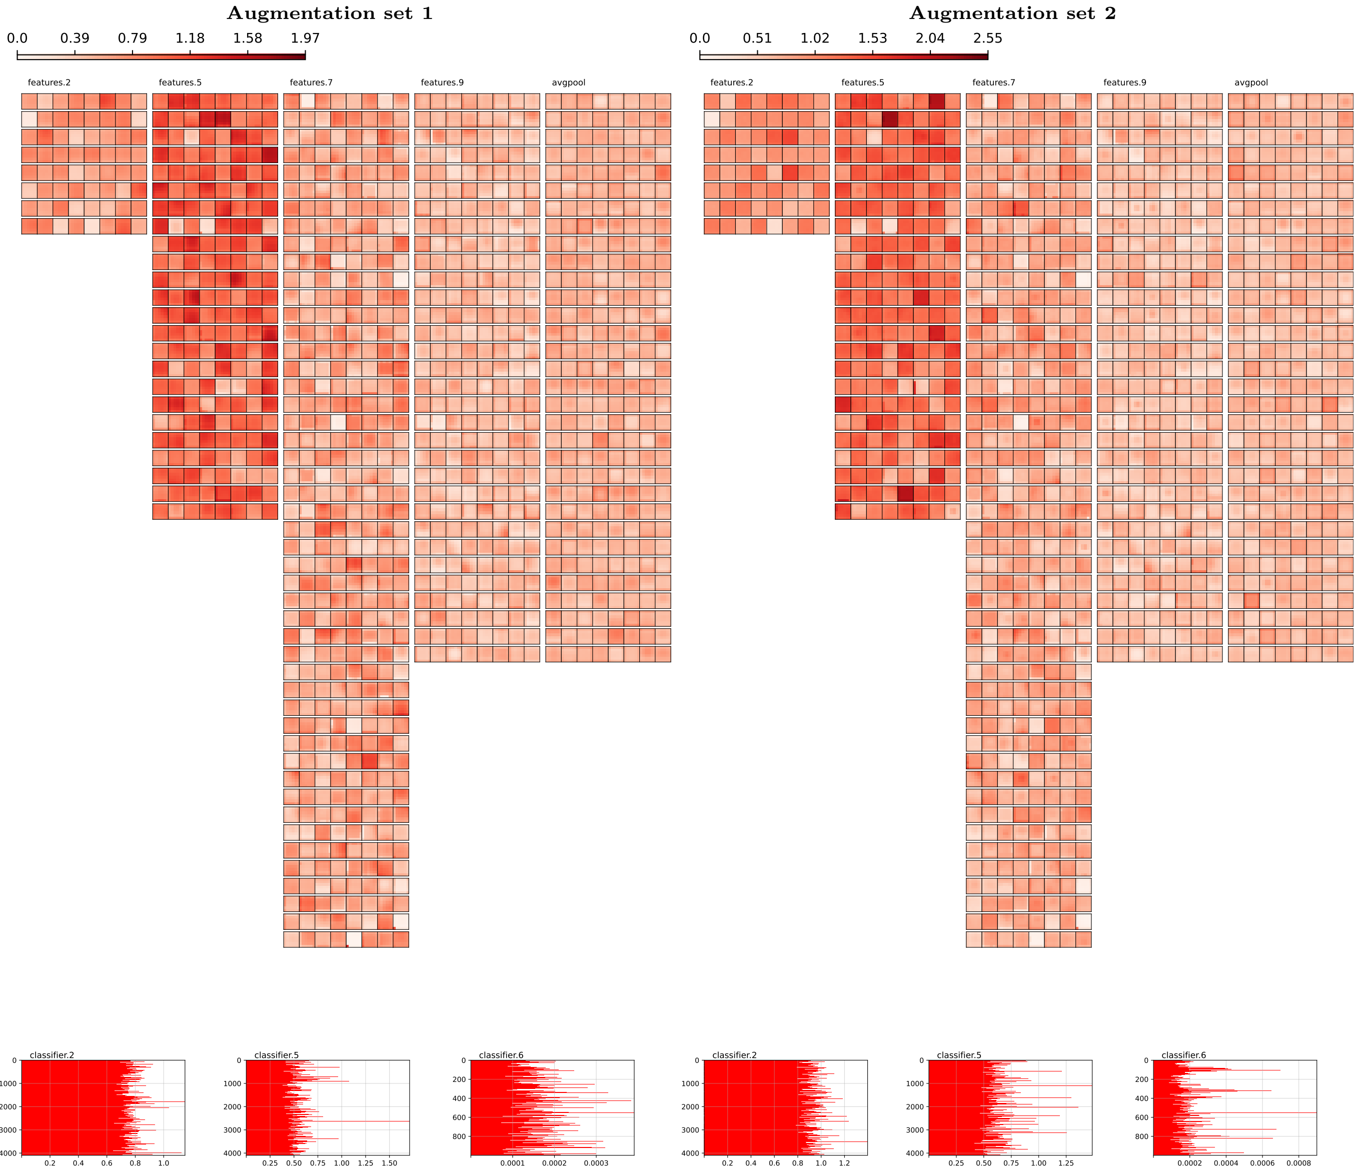


Figure S7.1.1 (b): Variances of activations plotted on a log scale ($\log_{10}(1+v)$). AlexNet network, Shapley values (sampling scheme 2).

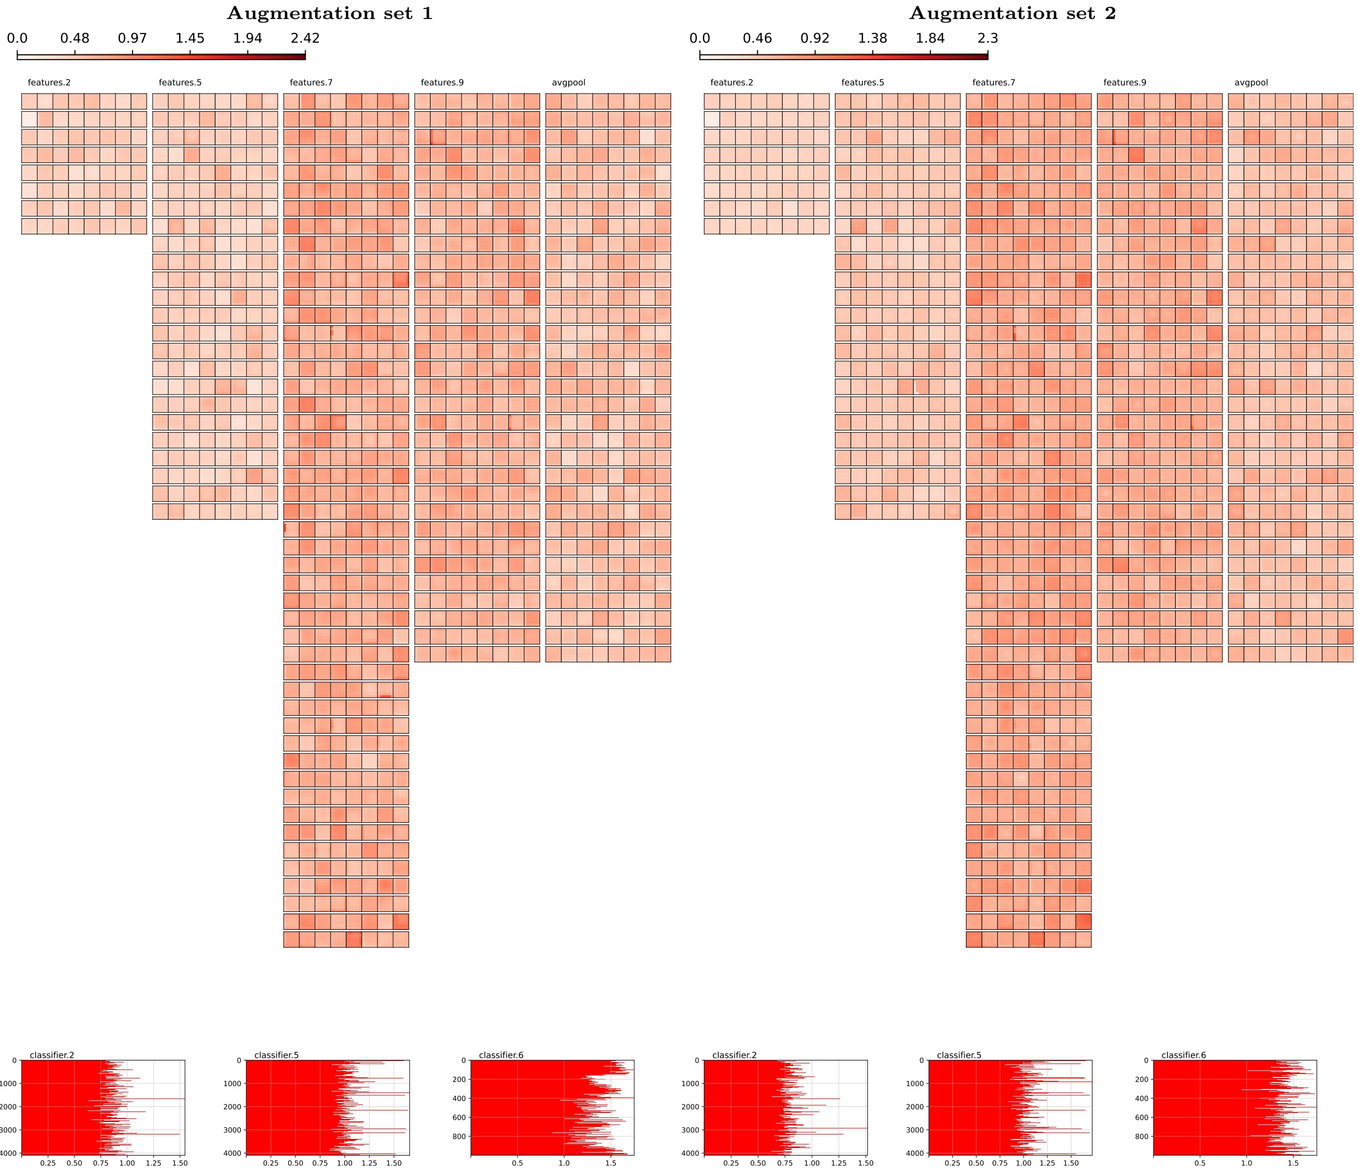


Figure S7.1.1 (c): Coefficients of variations of activations plotted on a log scale ($\log_{10}(1 + v)$). AlexNet network, Sobol indices (sampling scheme 1).

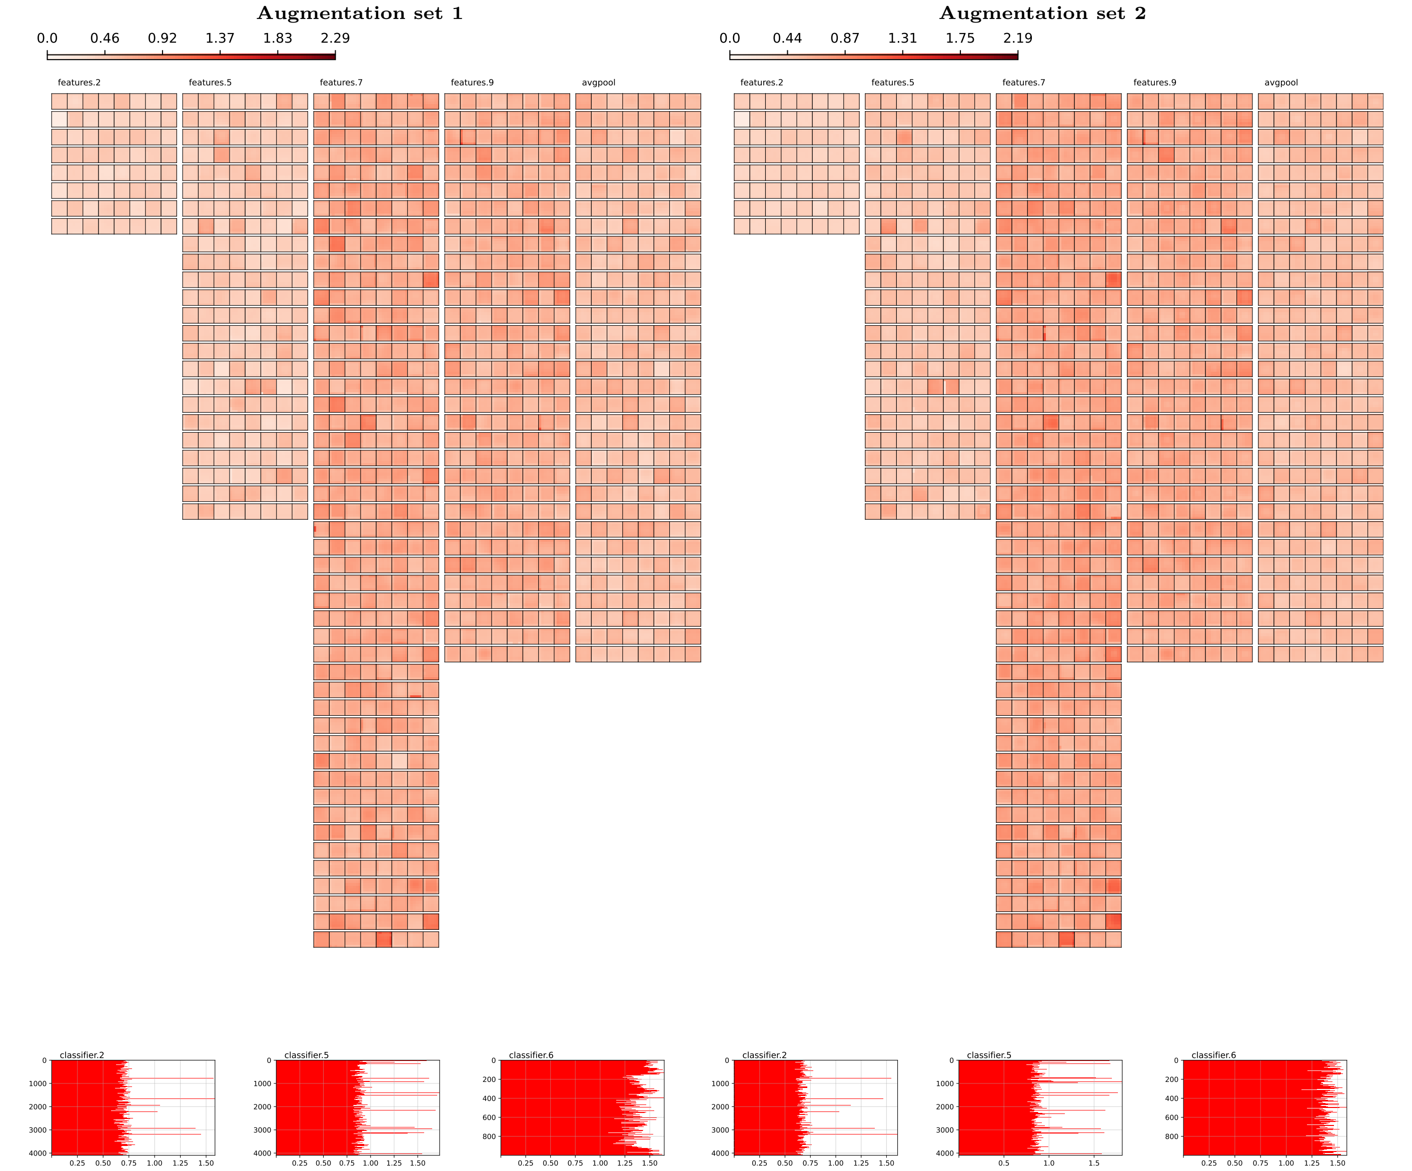


Figure S7.1.1 (d): Coefficients of variations of activations plotted on a log scale ($\log_{10}(1+v)$). AlexNet network, Shapley values (sampling scheme 2).

## 1.2 VGG11

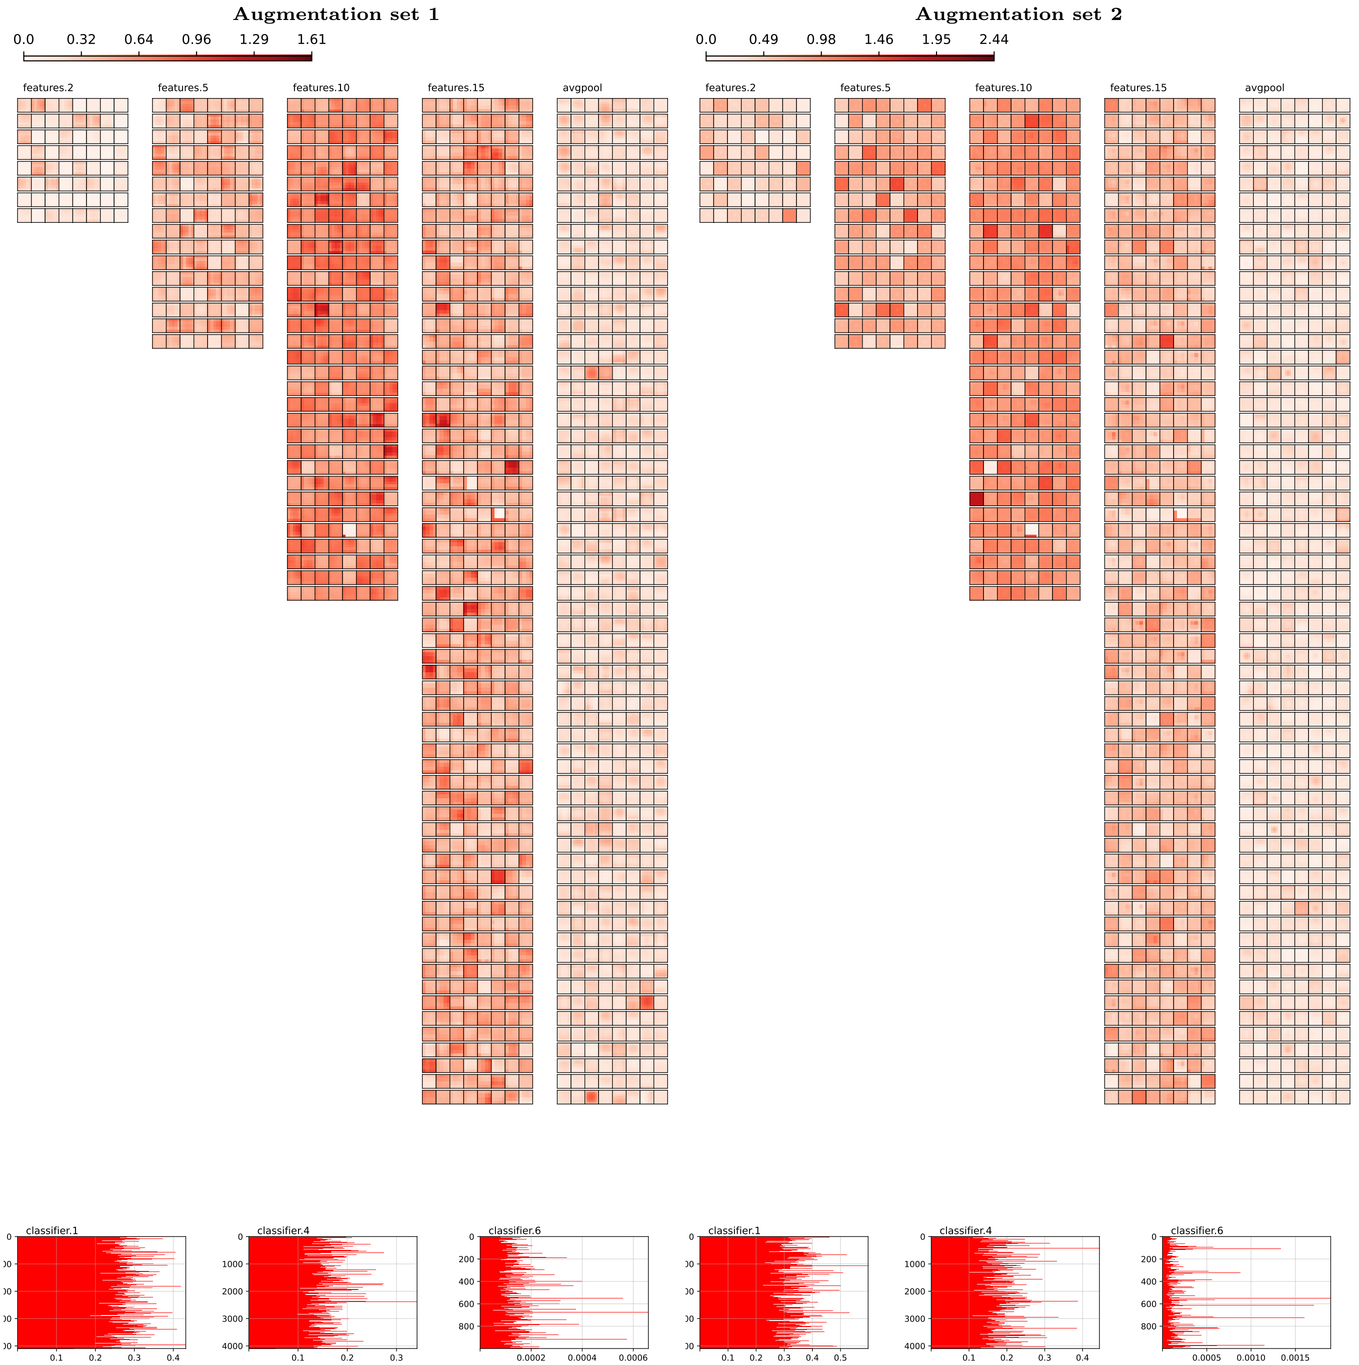


Figure S7.1.2 (a): Variances of activations plotted on a log scale ($\log_{10}(1 + v)$). VGG11 network, Sobol indices (sampling scheme 1).

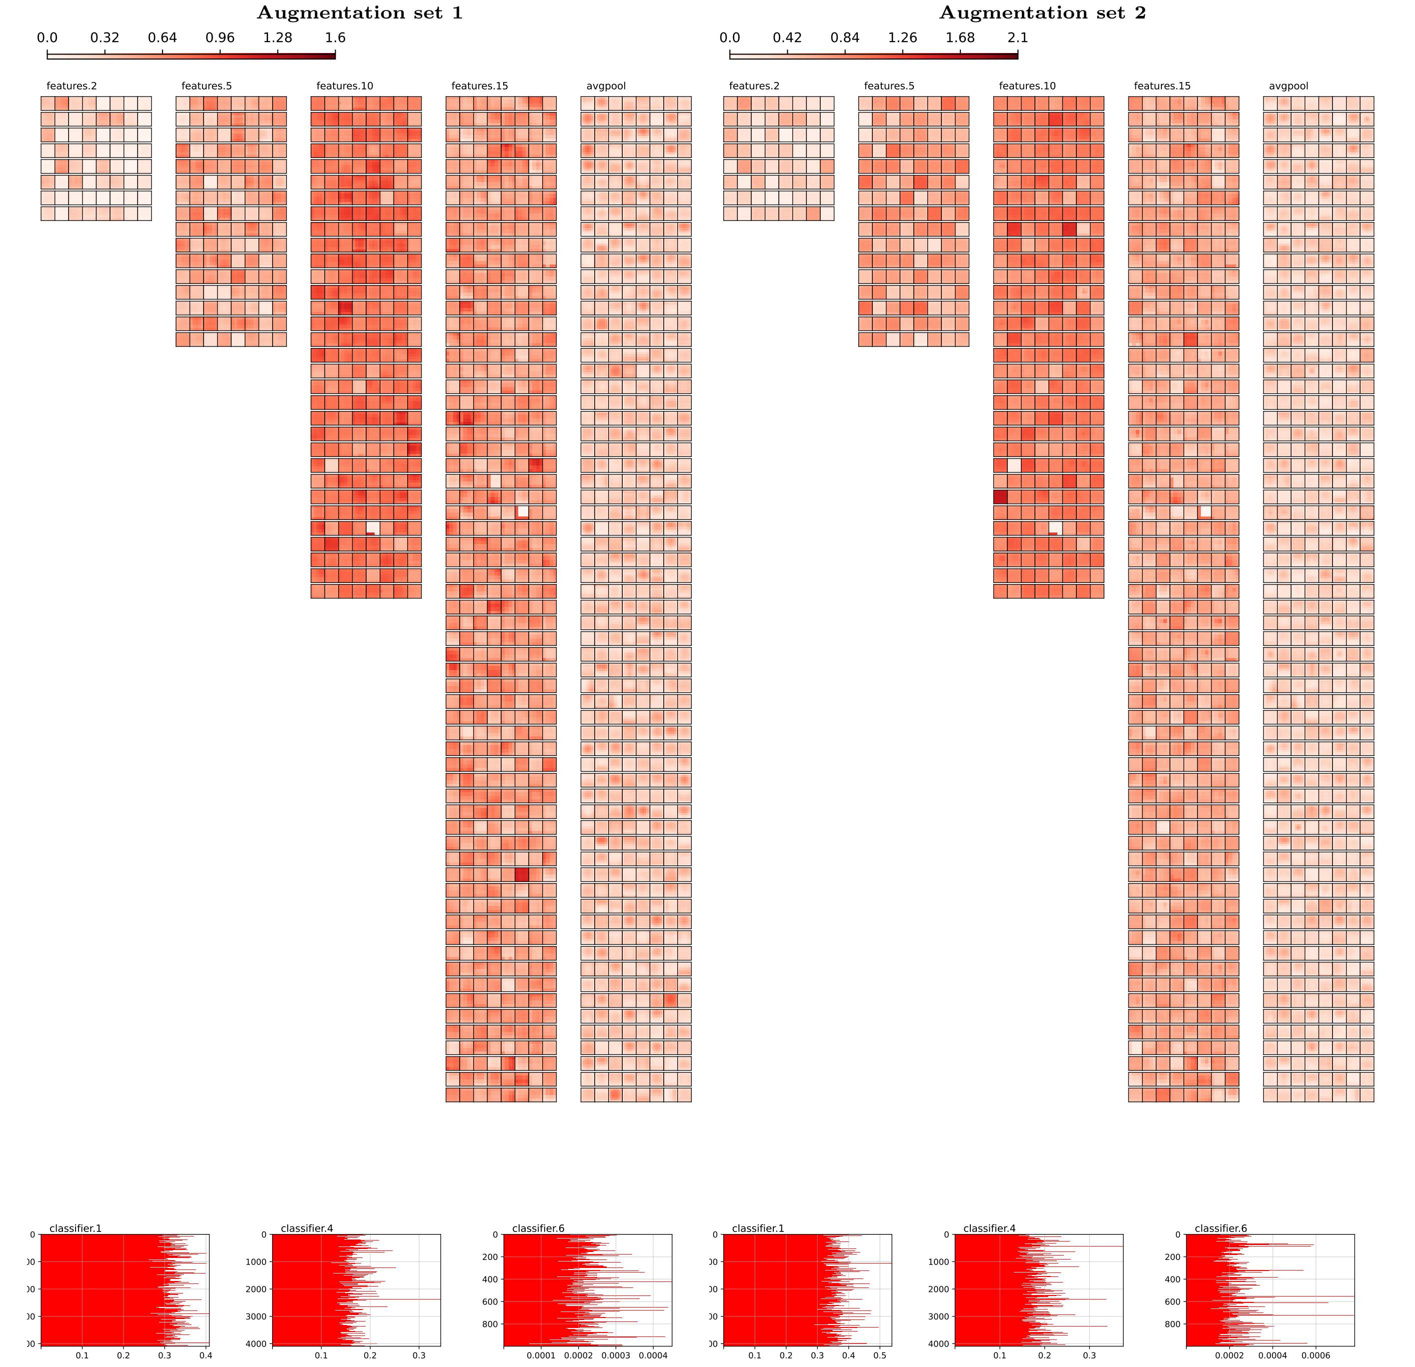


Figure S7.1.2 (b): Variances of activations plotted on a log scale ($\log_{10}(1+v)$). VGG11 network, Shapley values (sampling scheme 2).

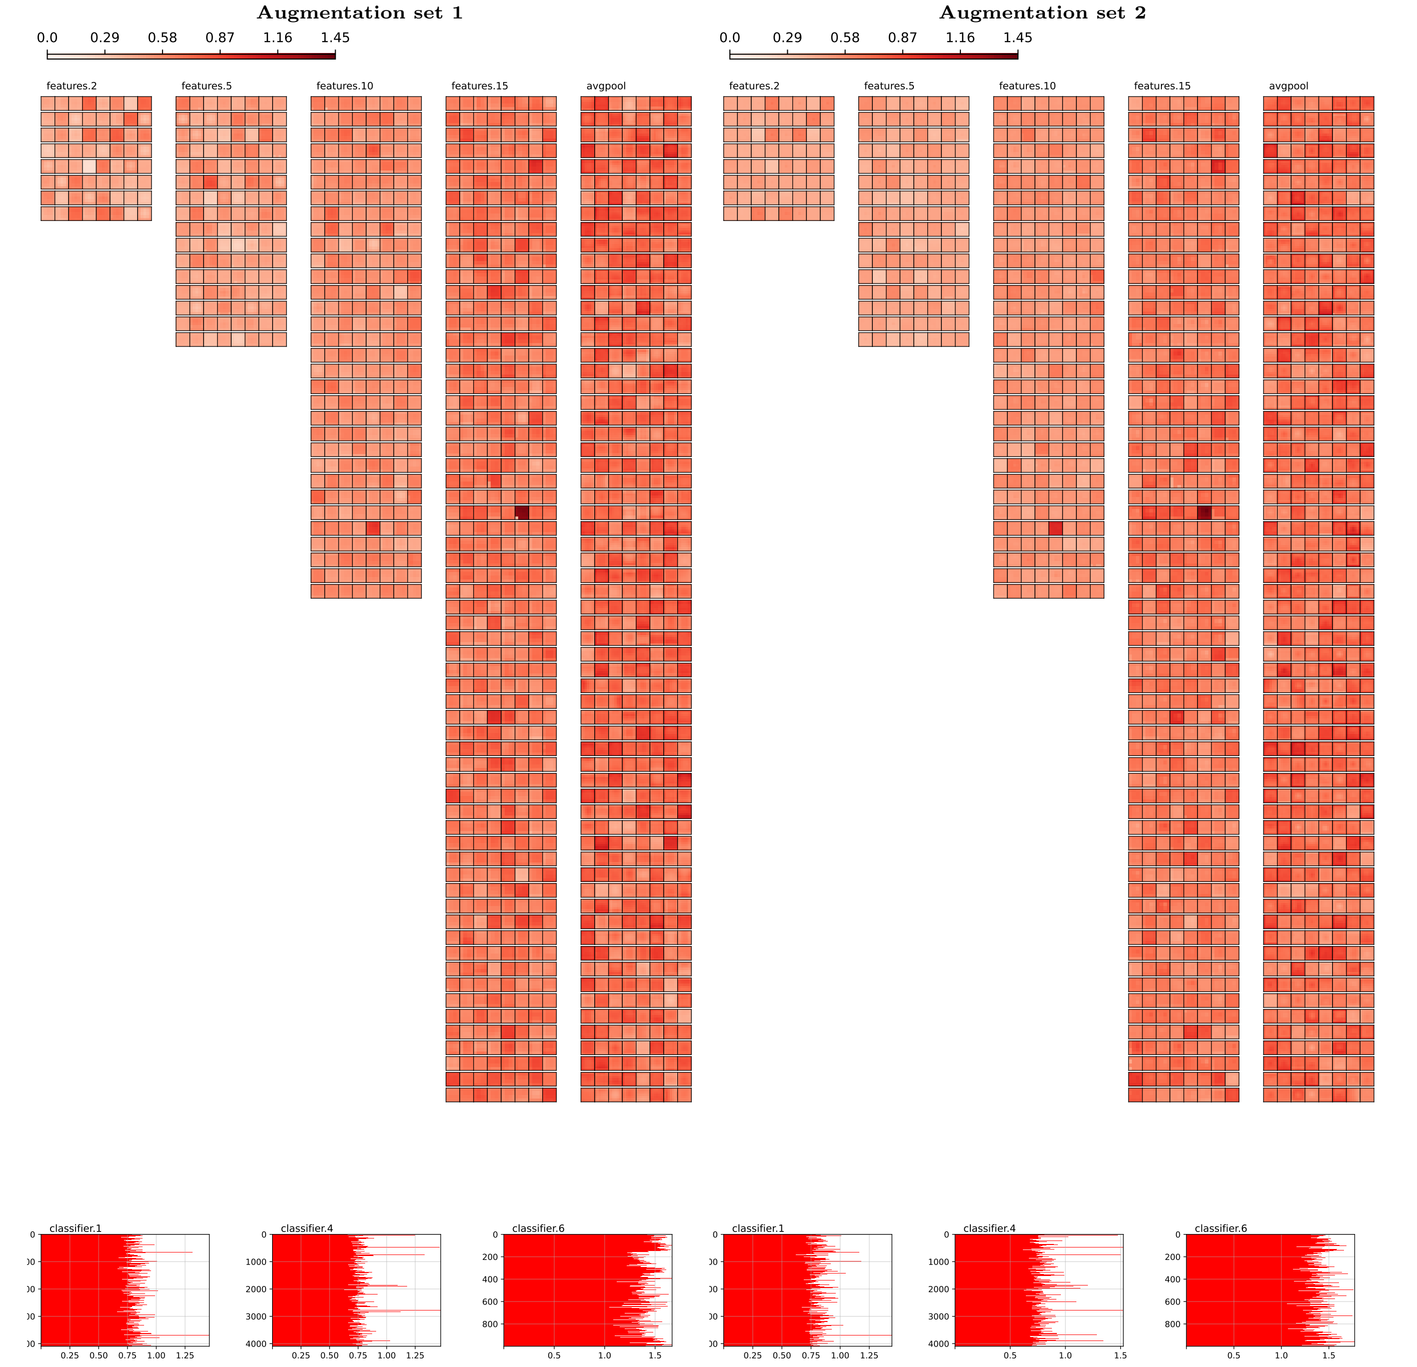


Figure S7.1.2 (c): Coefficients of variations of activations plotted on a log scale ($\log_{10}(1+v)$). VGG11 network, Sobol indices (sampling scheme 1).

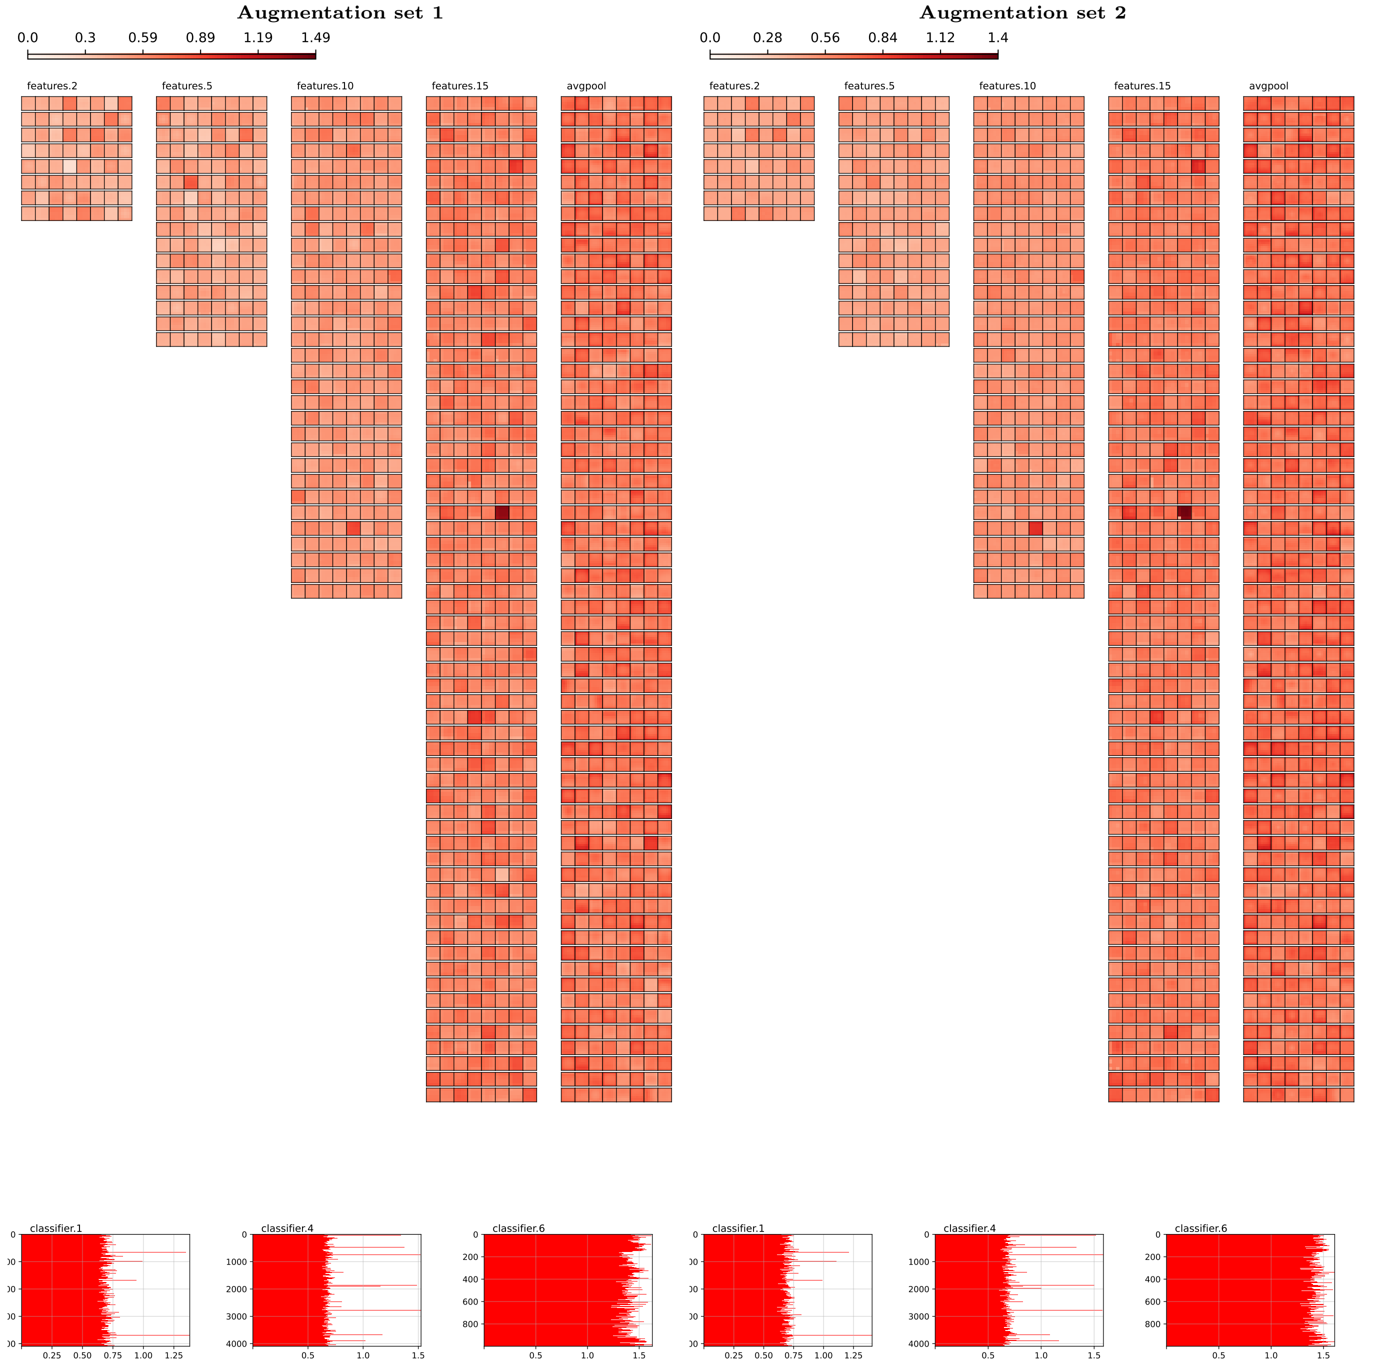


Figure S7.1.2 (d): Coefficients of variations of activations plotted on a log scale ($\log_{10}(1 + v)$). VGG11 network, Shapley values (sampling scheme 2).

## 1.3 ResNet18

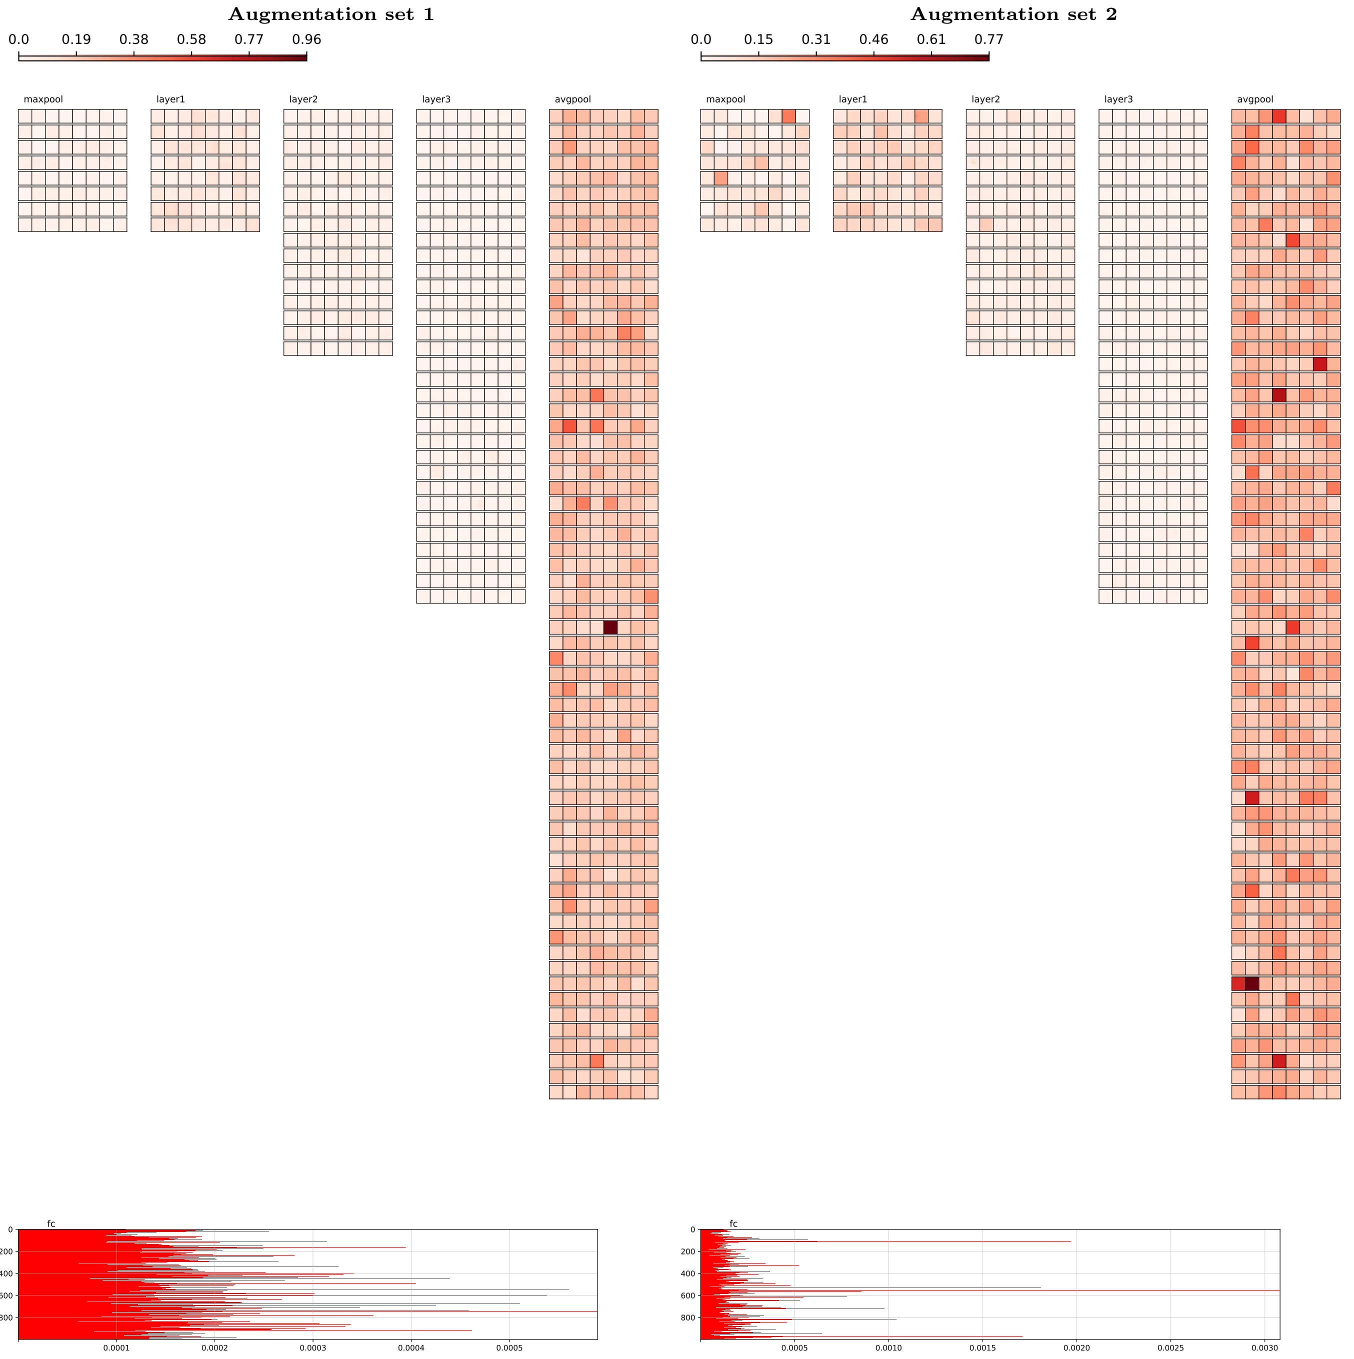


Figure S7.1.3 (a): Variances of activations plotted on a log scale ($\log_{10}(1+v)$). ResNet18 network, Sobol indices (sampling scheme 1).

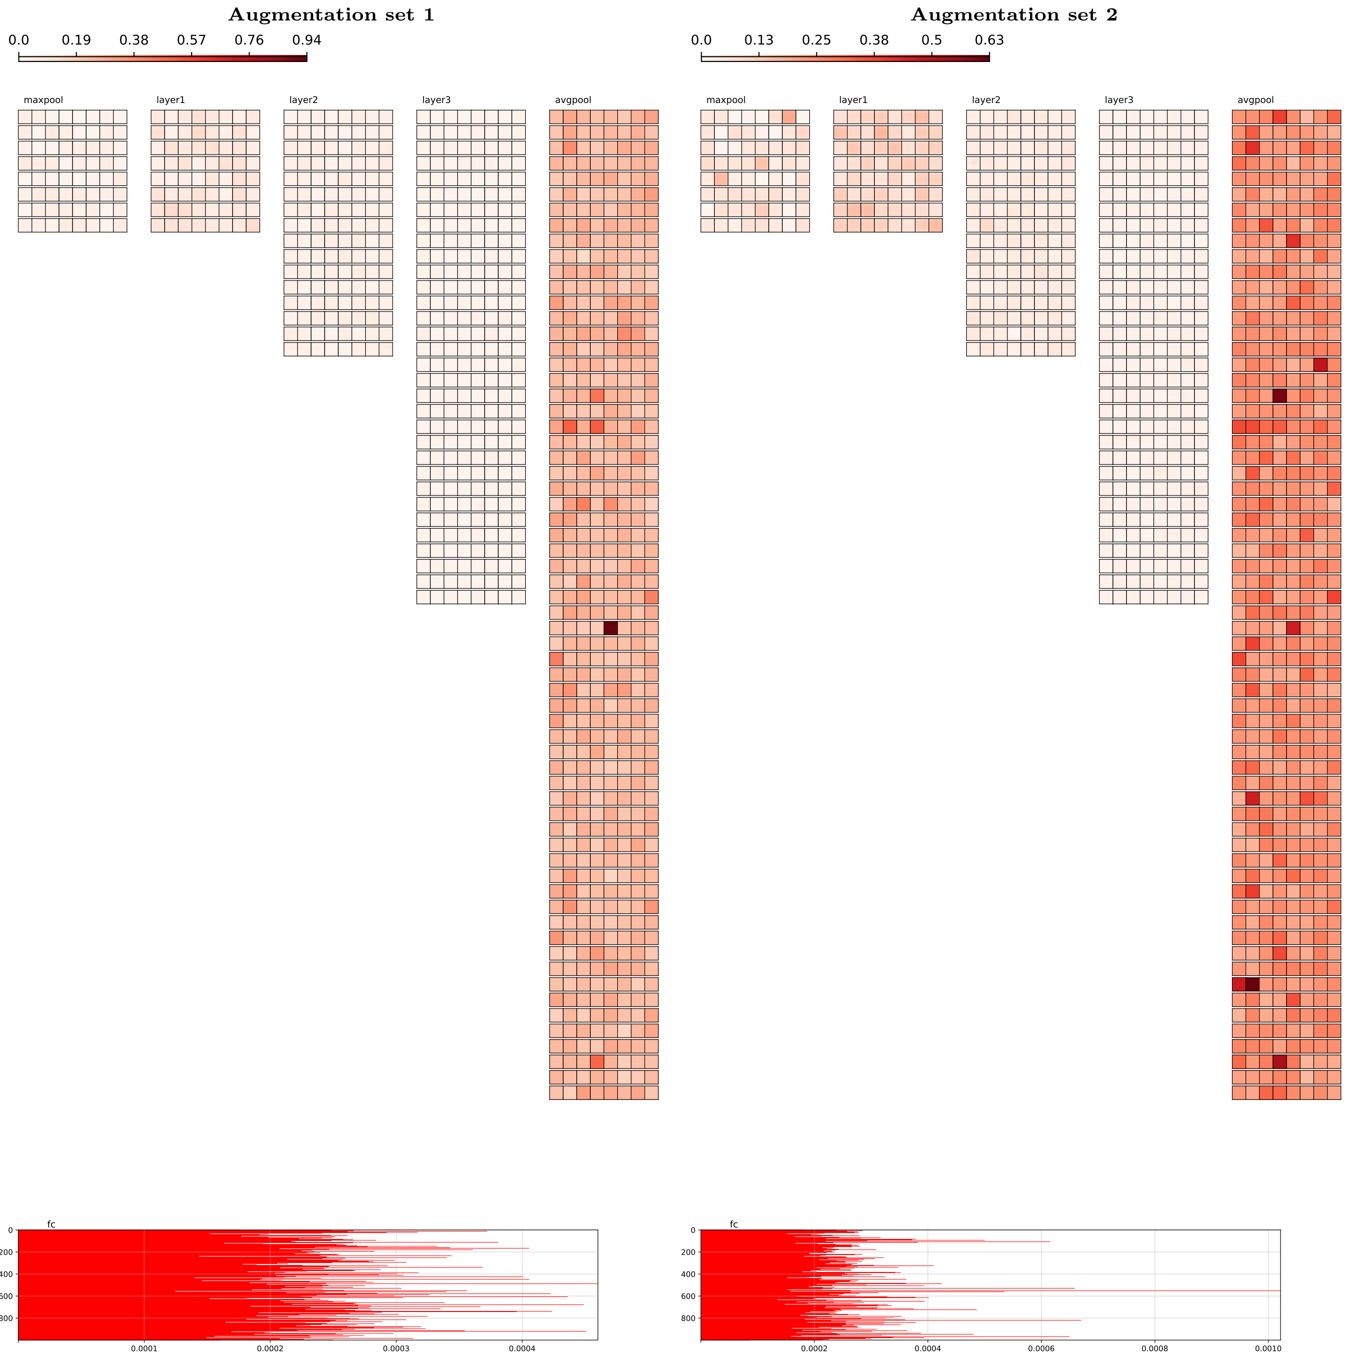


Figure S7.1.3 (b): Variances of activations plotted on a log scale ($\log_{10}(1 + v)$). ResNet18 network, Shapley values (sampling scheme 2).

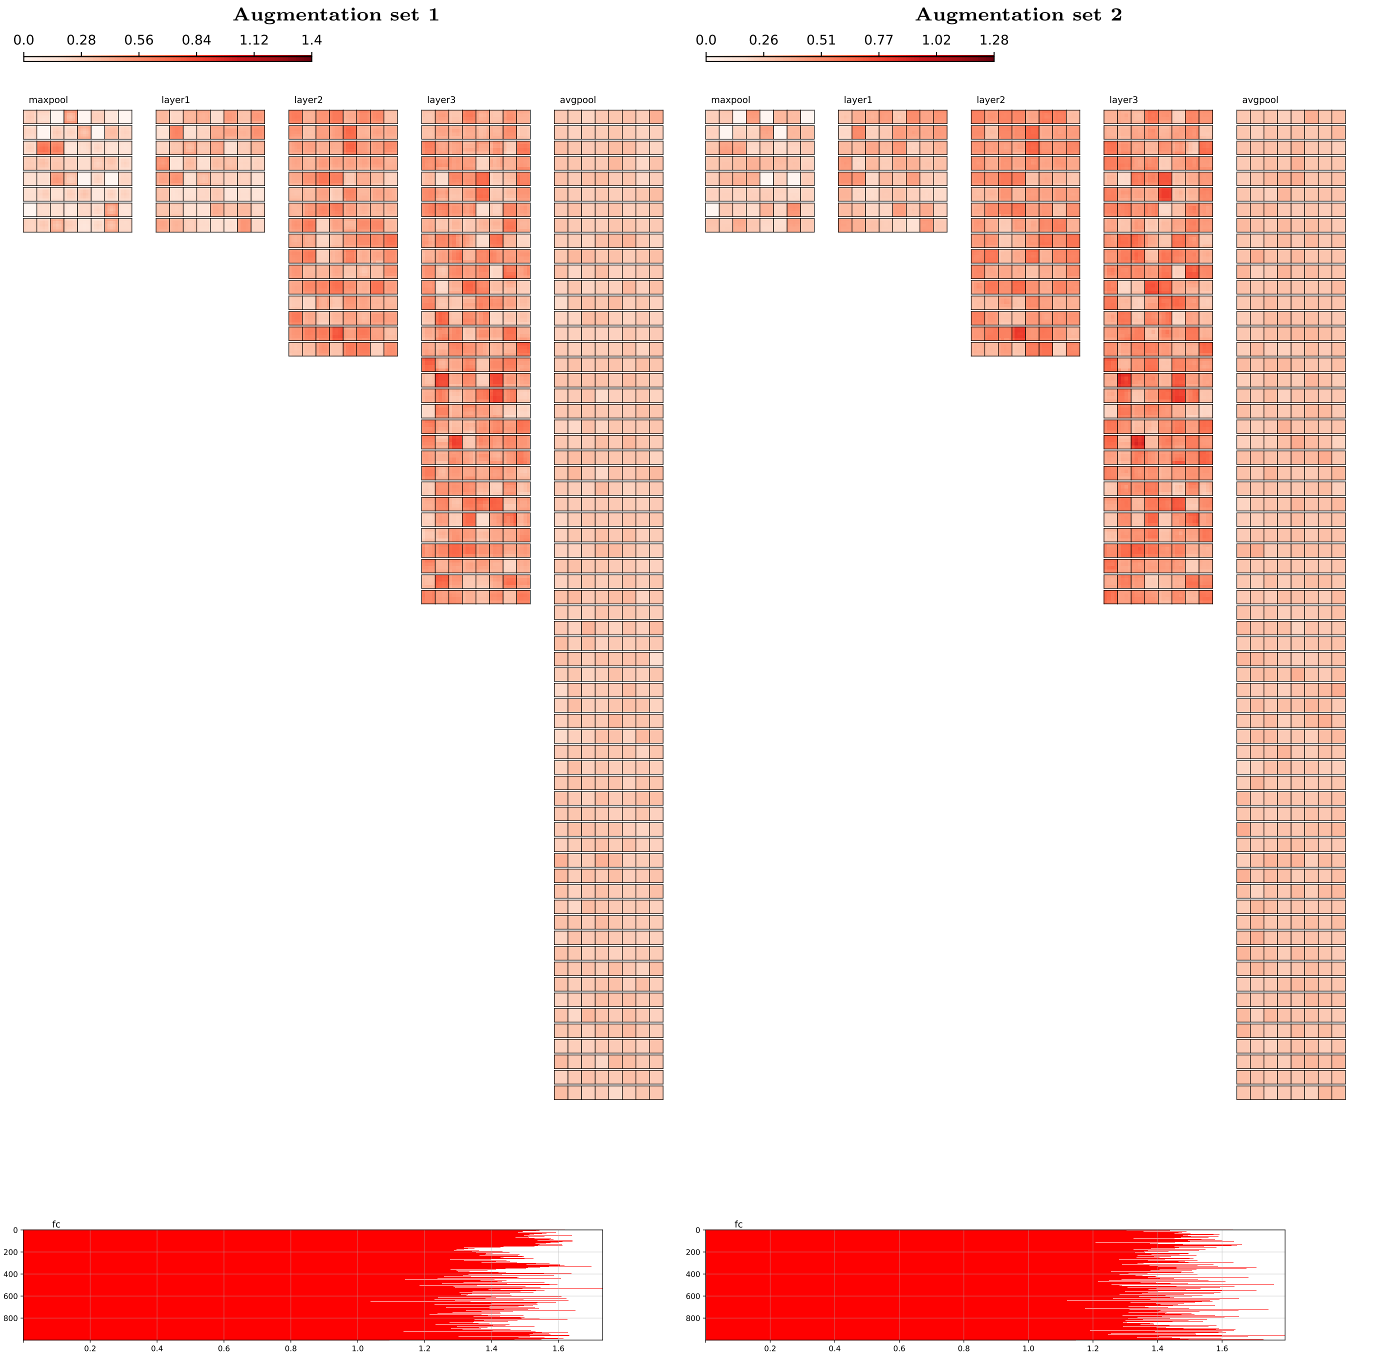


Figure S7.1.3 (c): Coefficients of variations of activations plotted on a log scale ($\log_{10}(1+v)$). ResNet18 network, Sobol indices (sampling scheme 1).

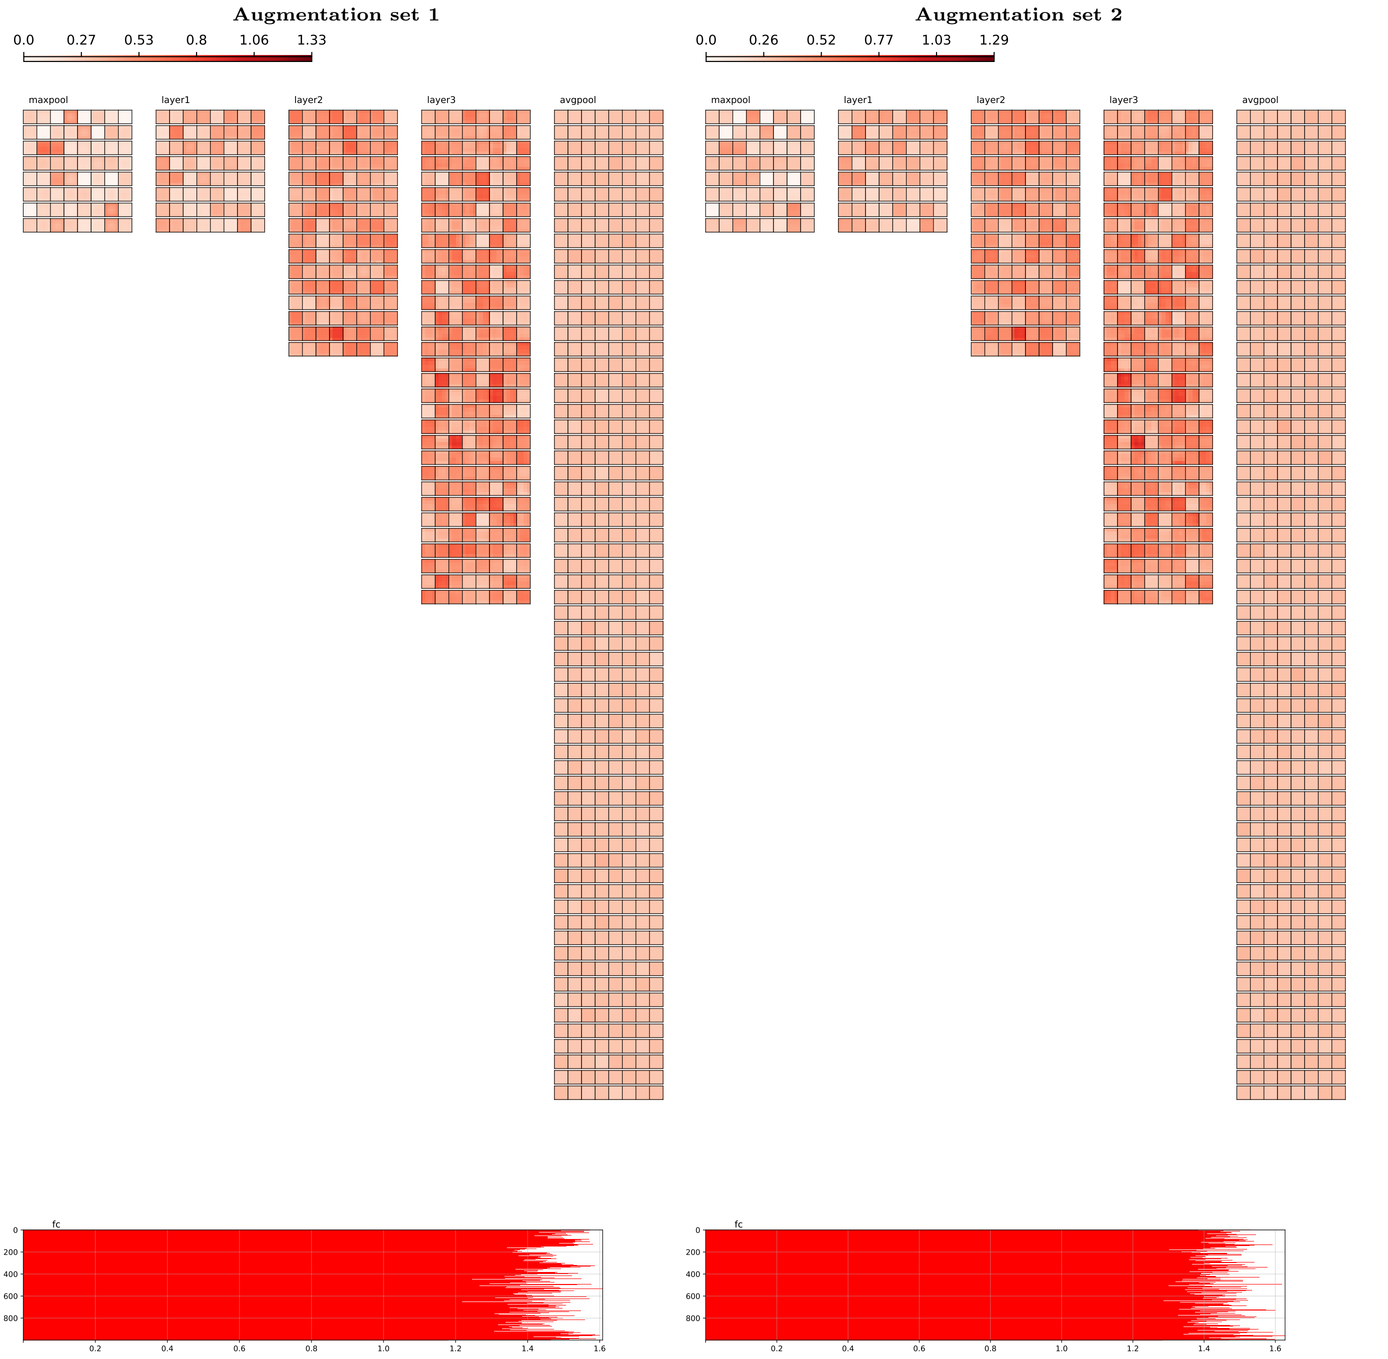


Figure S7.1.3 (d): Coefficients of variations of activations plotted on a log scale ($\log_{10}(1+v)$). ResNet18 network, Shapley values (sampling scheme 2).

# 2 Correlation between pairs of augmentation variables within selected sensitivity values

Full correlation matrices between sensitivity analysis variables used in both augmentation sets are depicted in Figures S7.2 (a)–S7.2 (e). All figures are divided into blocks according to the selected checkpoints (rows) and particular sensitivity values: rank biserial correlation coefficient measured on the training and validation partitions of the dataset (*rbscc (train)* and *rbscc (valid)*), Shapley values (*shpv*), the first-order Sobol indices (*si*), and the total Sobol indices (*siT*).

To analyze the inner components of the network, one may consider a pairwise comparison of their outputs computed either augmenting the input or not, e.g., in terms of a rank biserial correlation coefficient (RBSCC) as a metric reflecting the impact on a fixed activation. However, within this framework, it is impossible to incorporate the impact of multiple simultaneous transforms and auxiliary variables related to data and define connections between variables (e.g., the order in which transforms are to be applied). Another notable drawback is that the values are ideally correlated between treatments from both augmentation sets depending only on their number, indicating the high impact of original data diminishing any other relationships. Thus further research was designed on the basis of a direct variance analysis in terms of sensitivity values, which assess the extent of the impact of each variable on the total variances.

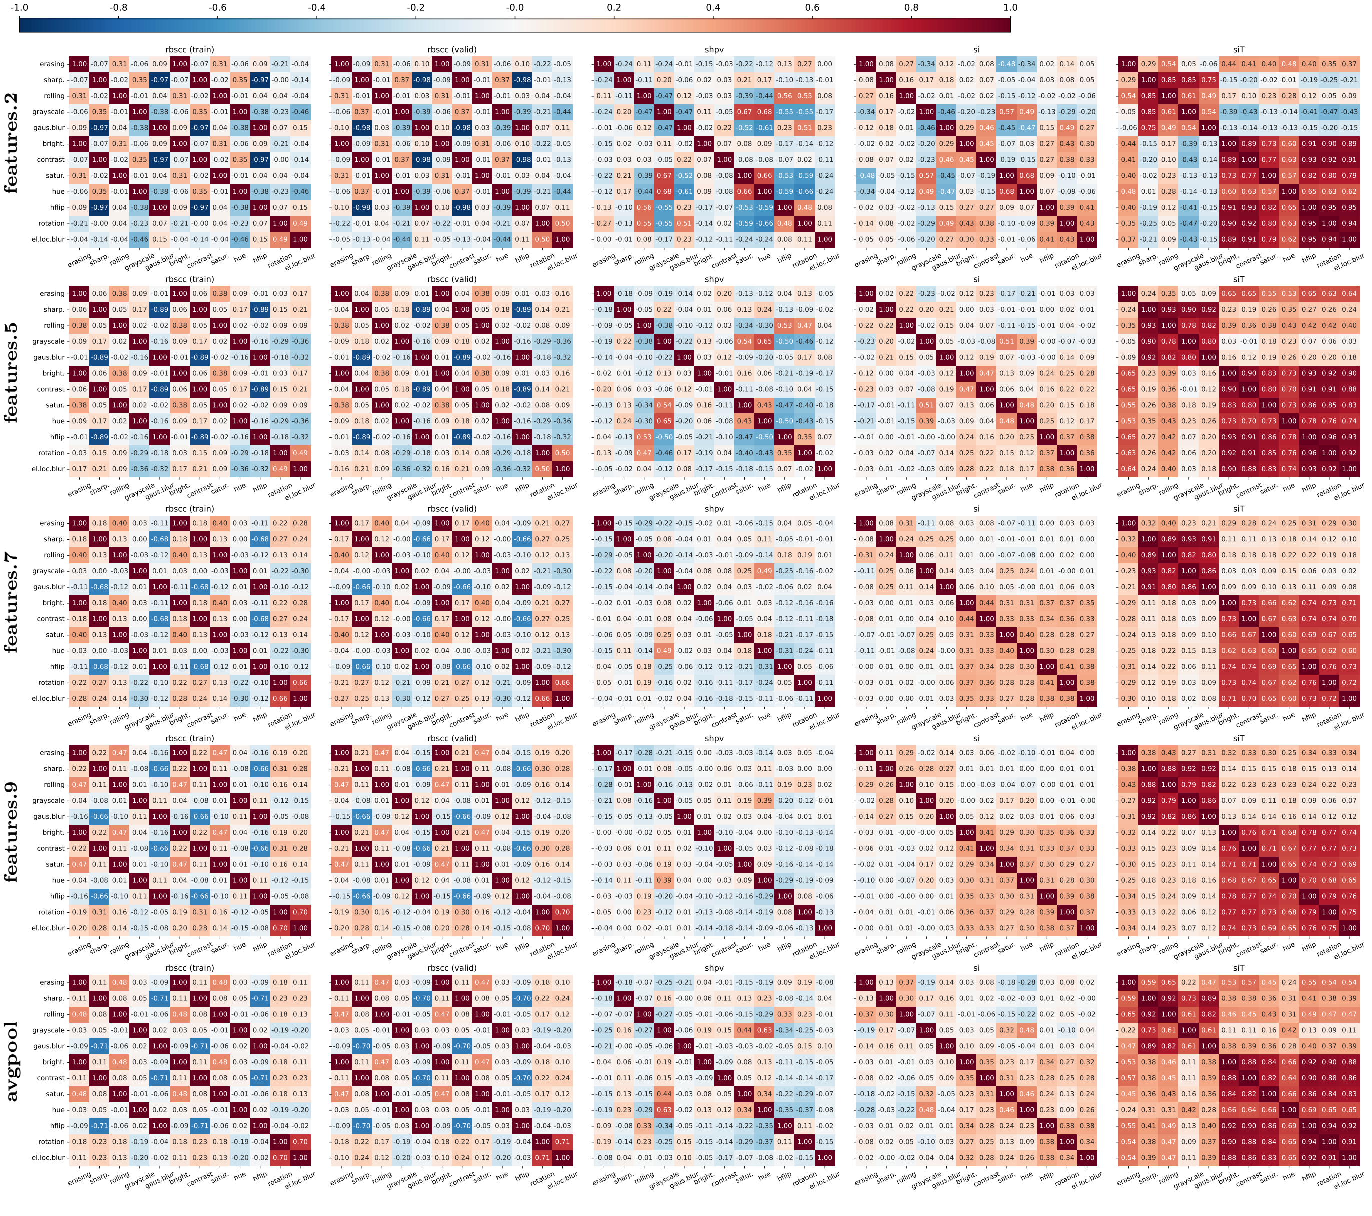


Figure S7.2 (a): Correlation between pairs of augmentation variables for convolutional checkpoints of AlexNet.

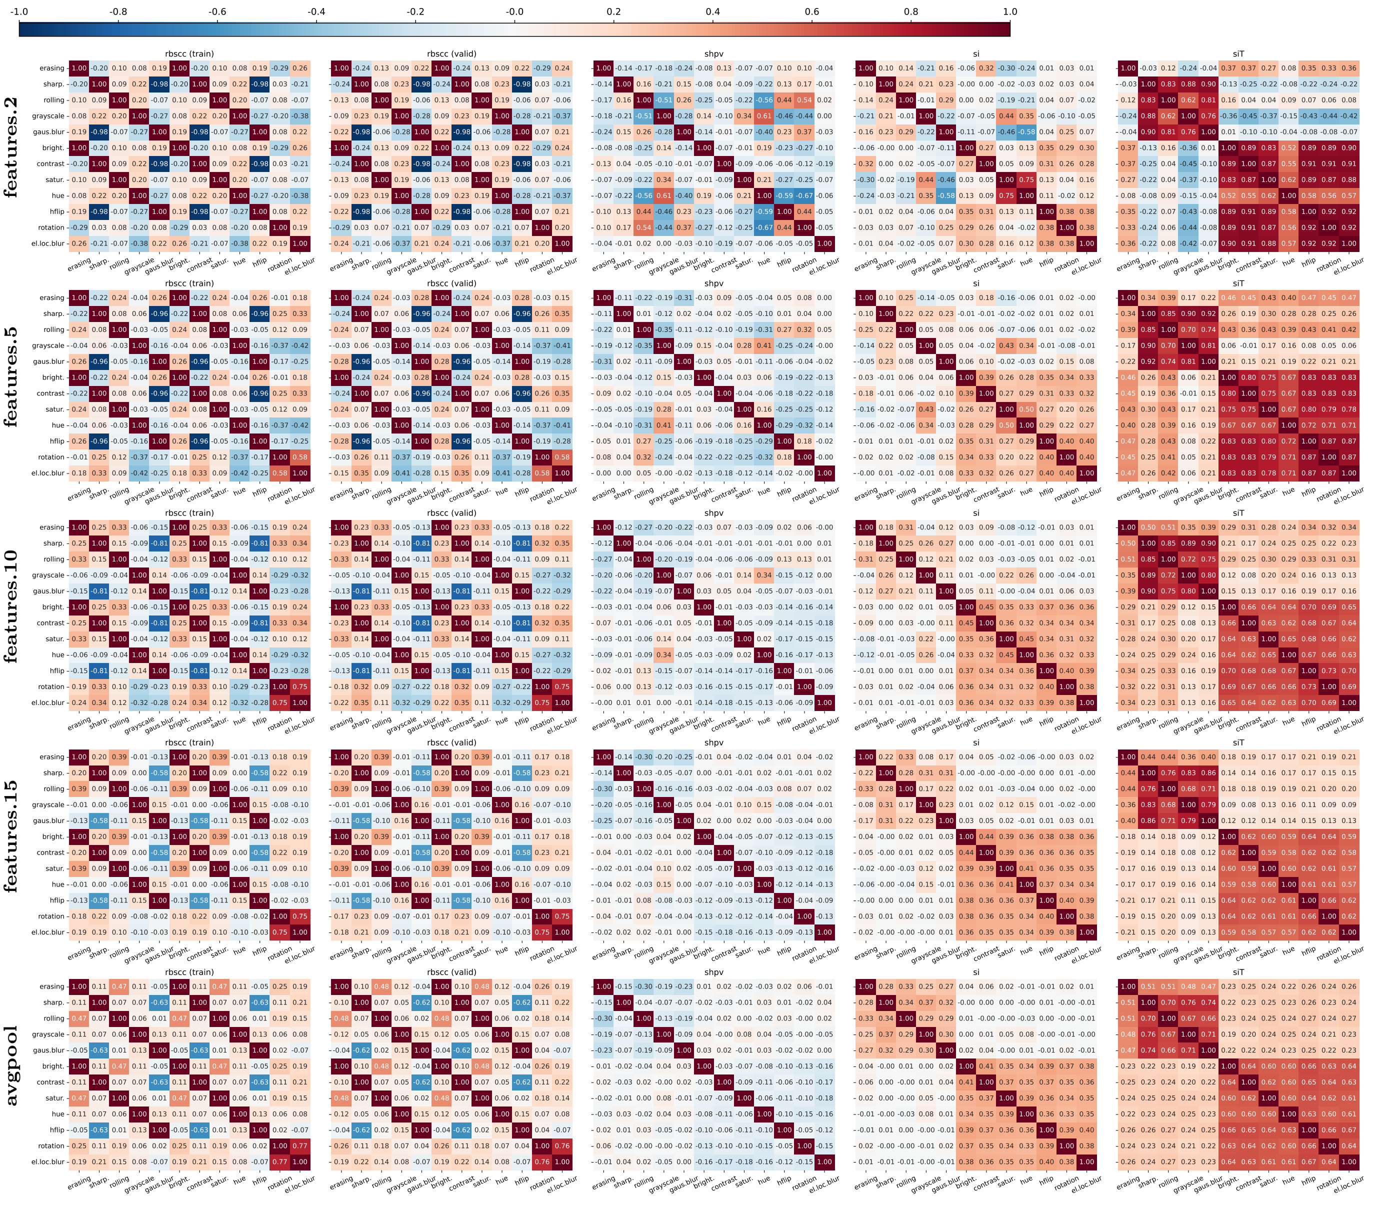


Figure S7.2 (b): Correlation between pairs of augmentation variables for convolutional checkpoints of VGG11.

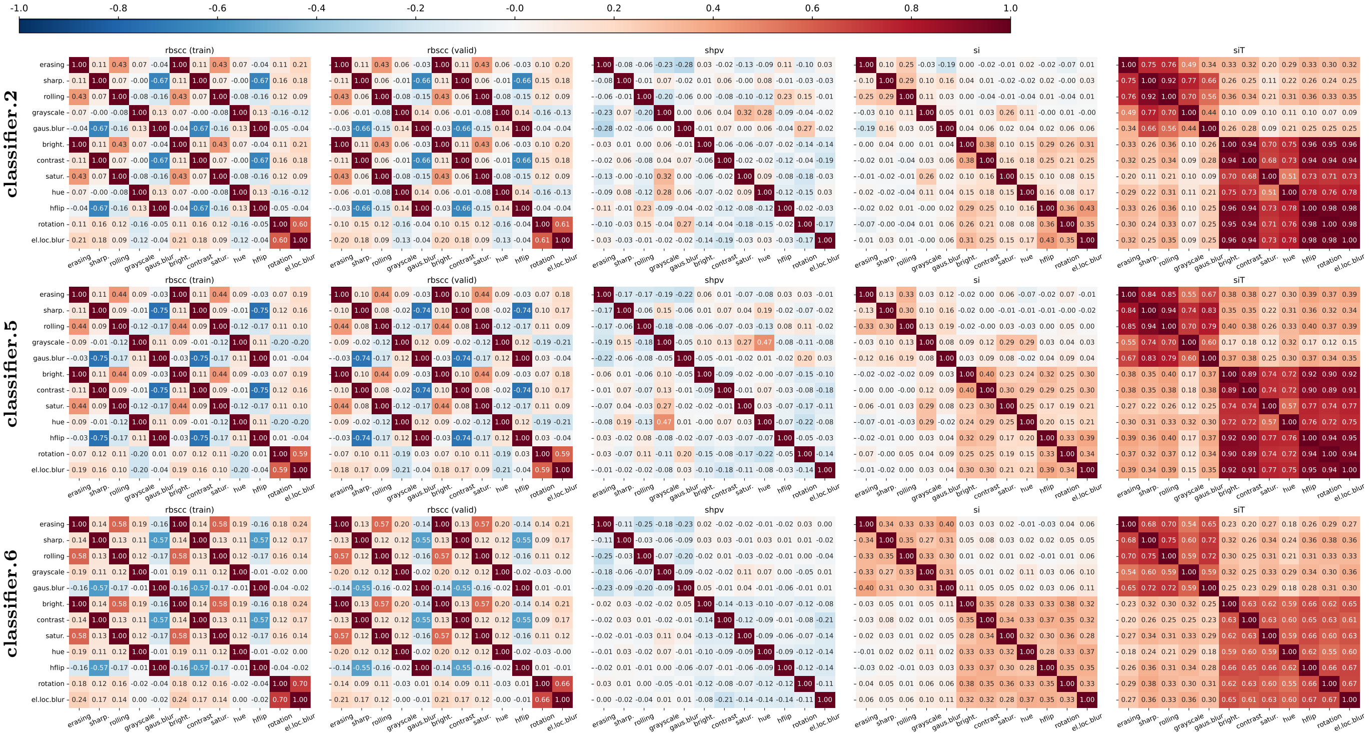


Figure S7.2 (c): Correlation between pairs of augmentation variables for fully-connected checkpoints of AlexNet.

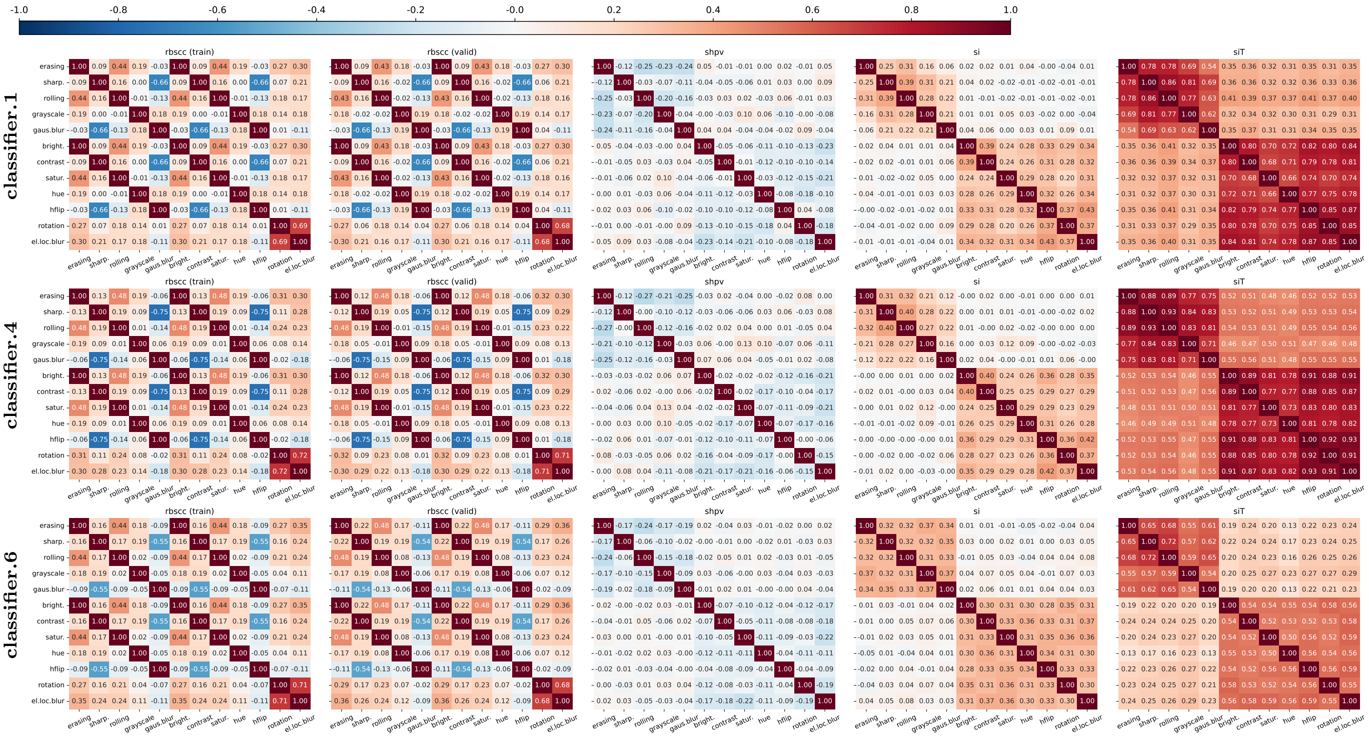


Figure S7.2 (d): Correlation between pairs of augmentation variables for fully-connected checkpoints of VGG11.

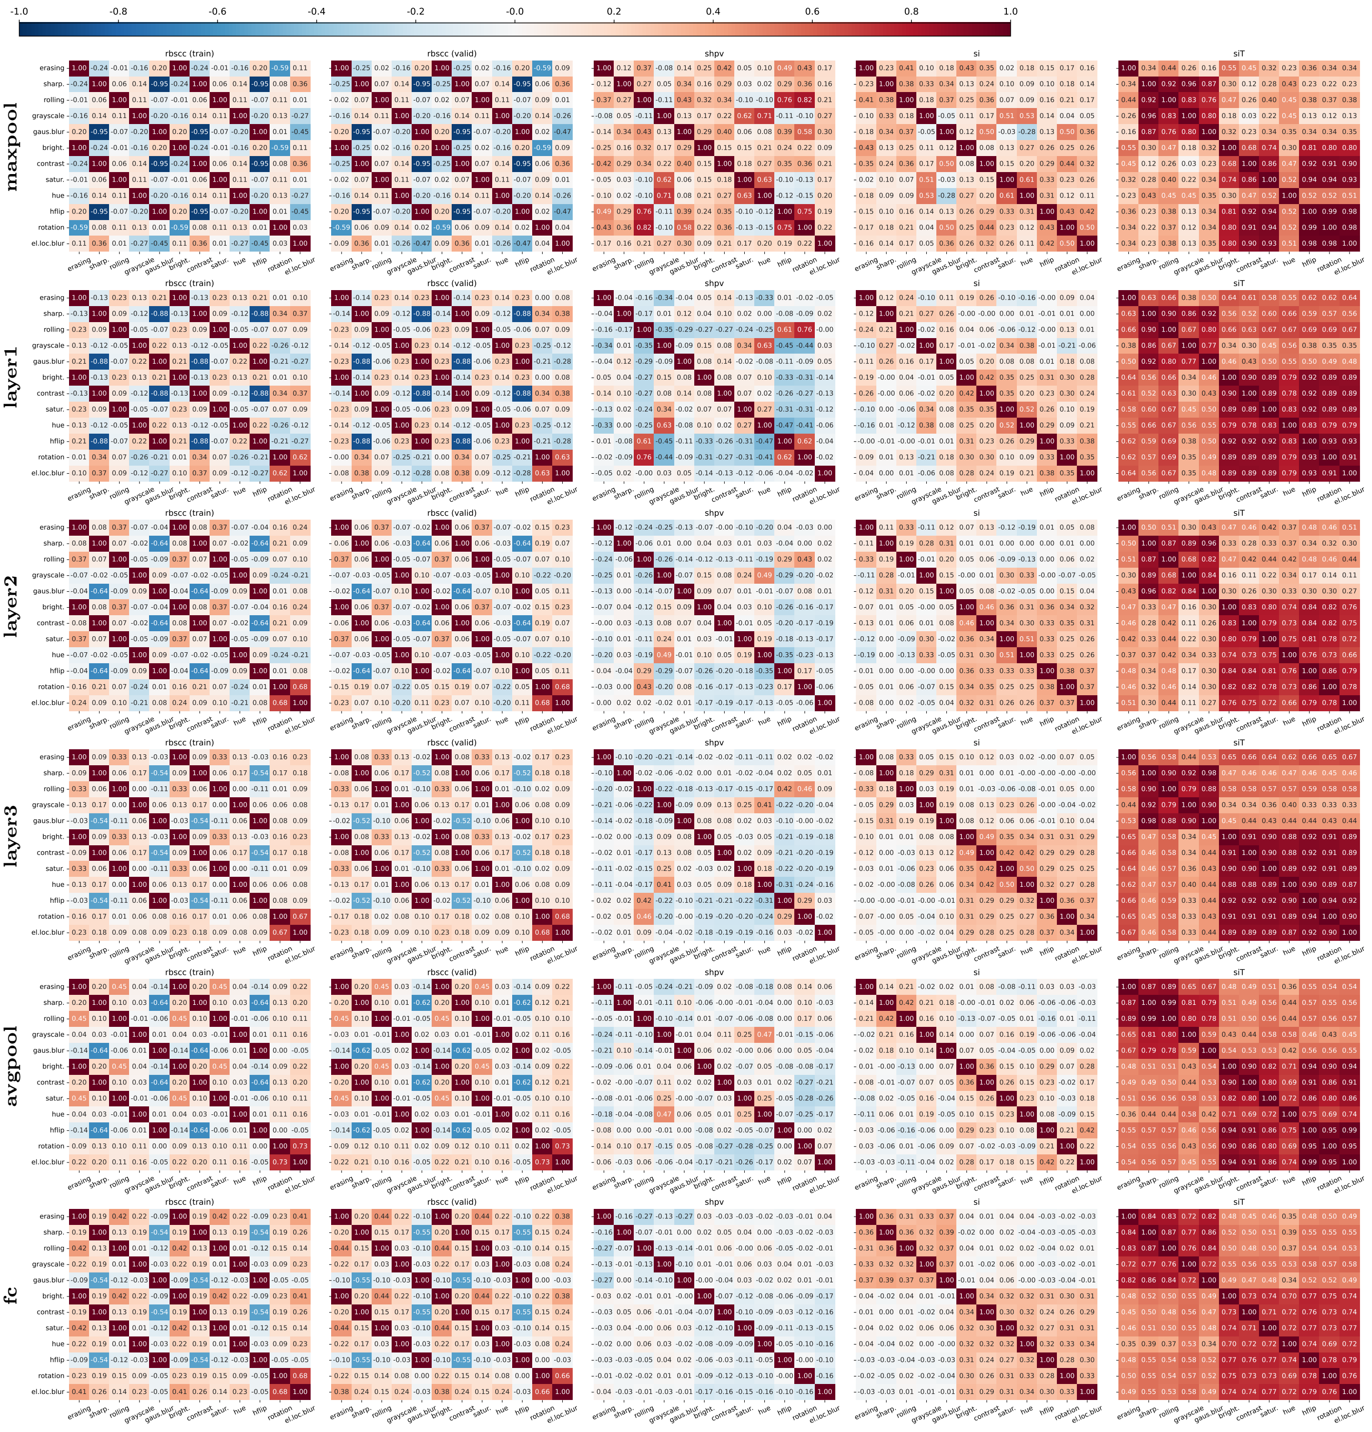


Figure S7.2 (e): Correlation between pairs of augmentation variables for convolutional and fully-conected checkpoints of ResNet18.

# 3 Spatial maps for unit-wise correlations between sensitivities and coefficients of variation

Figures S7.3 (a)–S7.3 (c) are separated into horizontal blocks assigned to the network's checkpoints selected for sensitivity analysis in this study. The corresponding name of a checkpoint is given on the left of a block. The rows of a single block are related to different sensitivity values: Shapley values (*shpv*), the first-order Sobol indices (*si*), and the total Sobol indices (*siT*). Columns of these blocks represent SA variables. The first augmentation set's variables are listed first, followed by ones from the second set.

These figures contain images for both convolutional and fully-connected checkpoints. It should be noted that the map is a single number for fully-connected checkpoints.

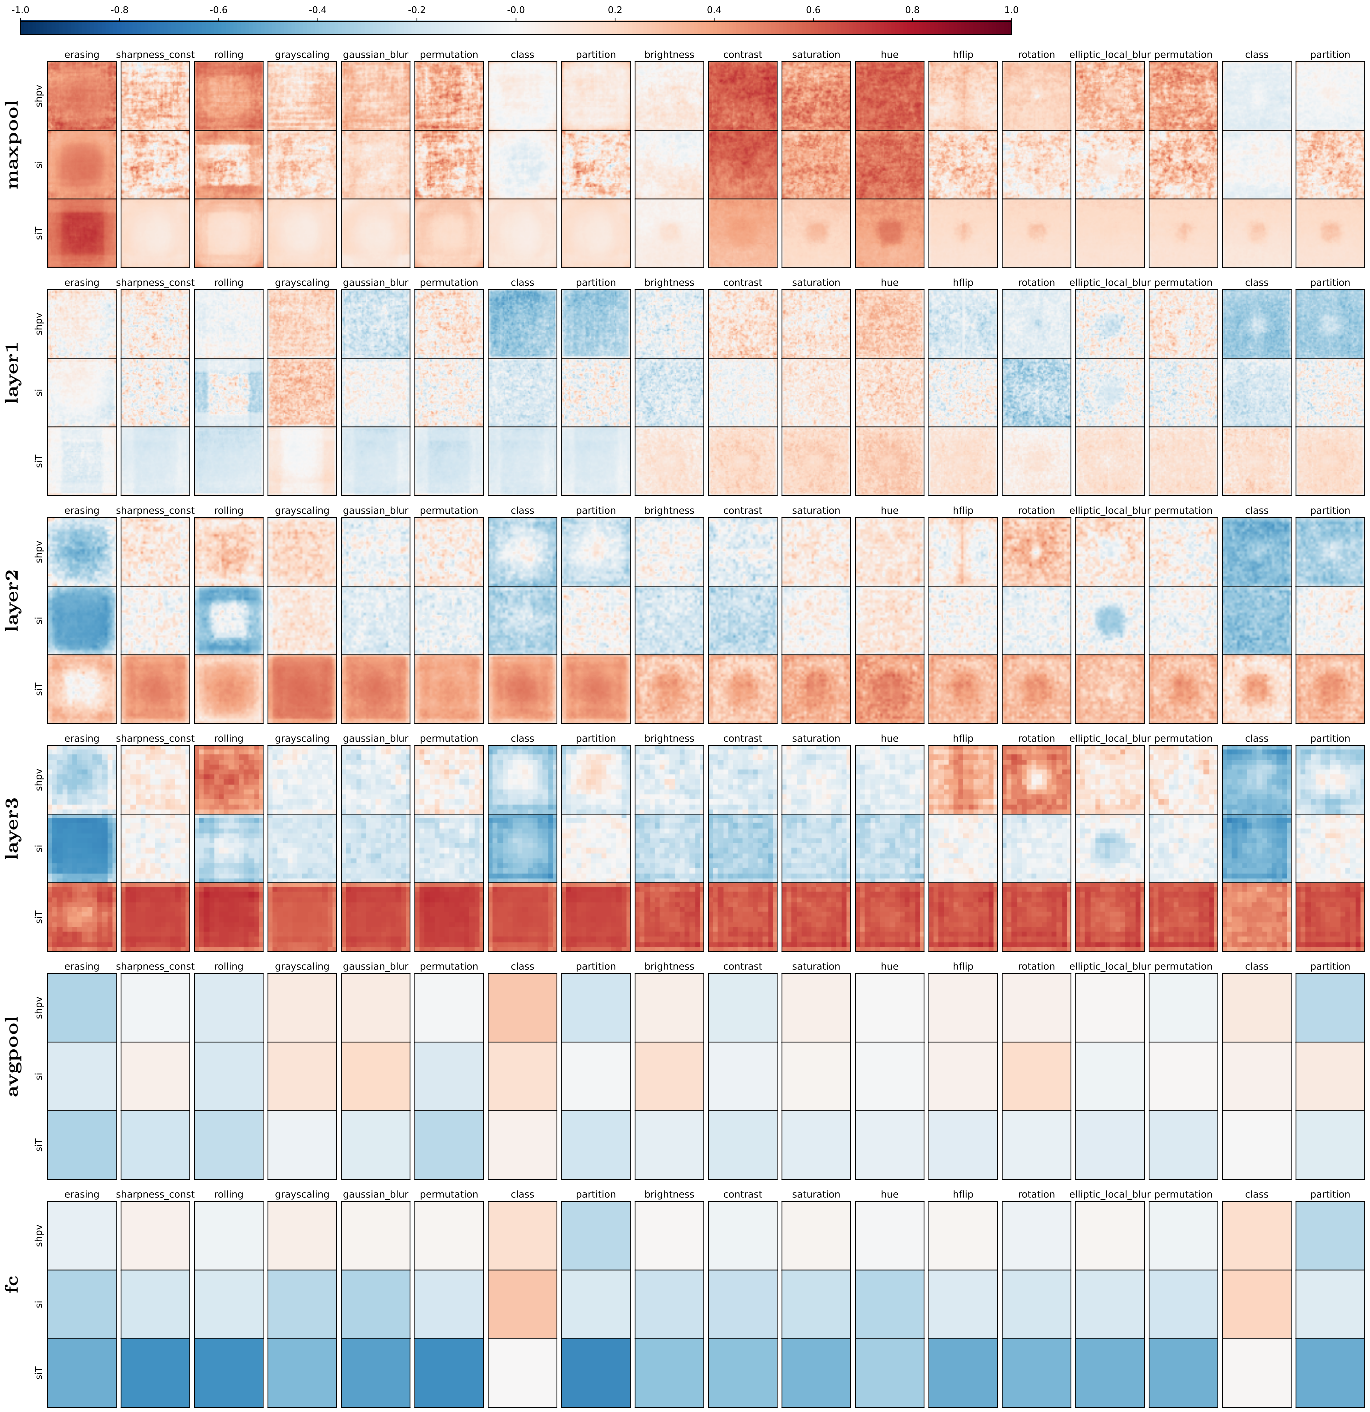


Figure S7.3 (a): Spatial maps for unit-wise correlations between sensitivities and coefficients of variation (ResNet18).

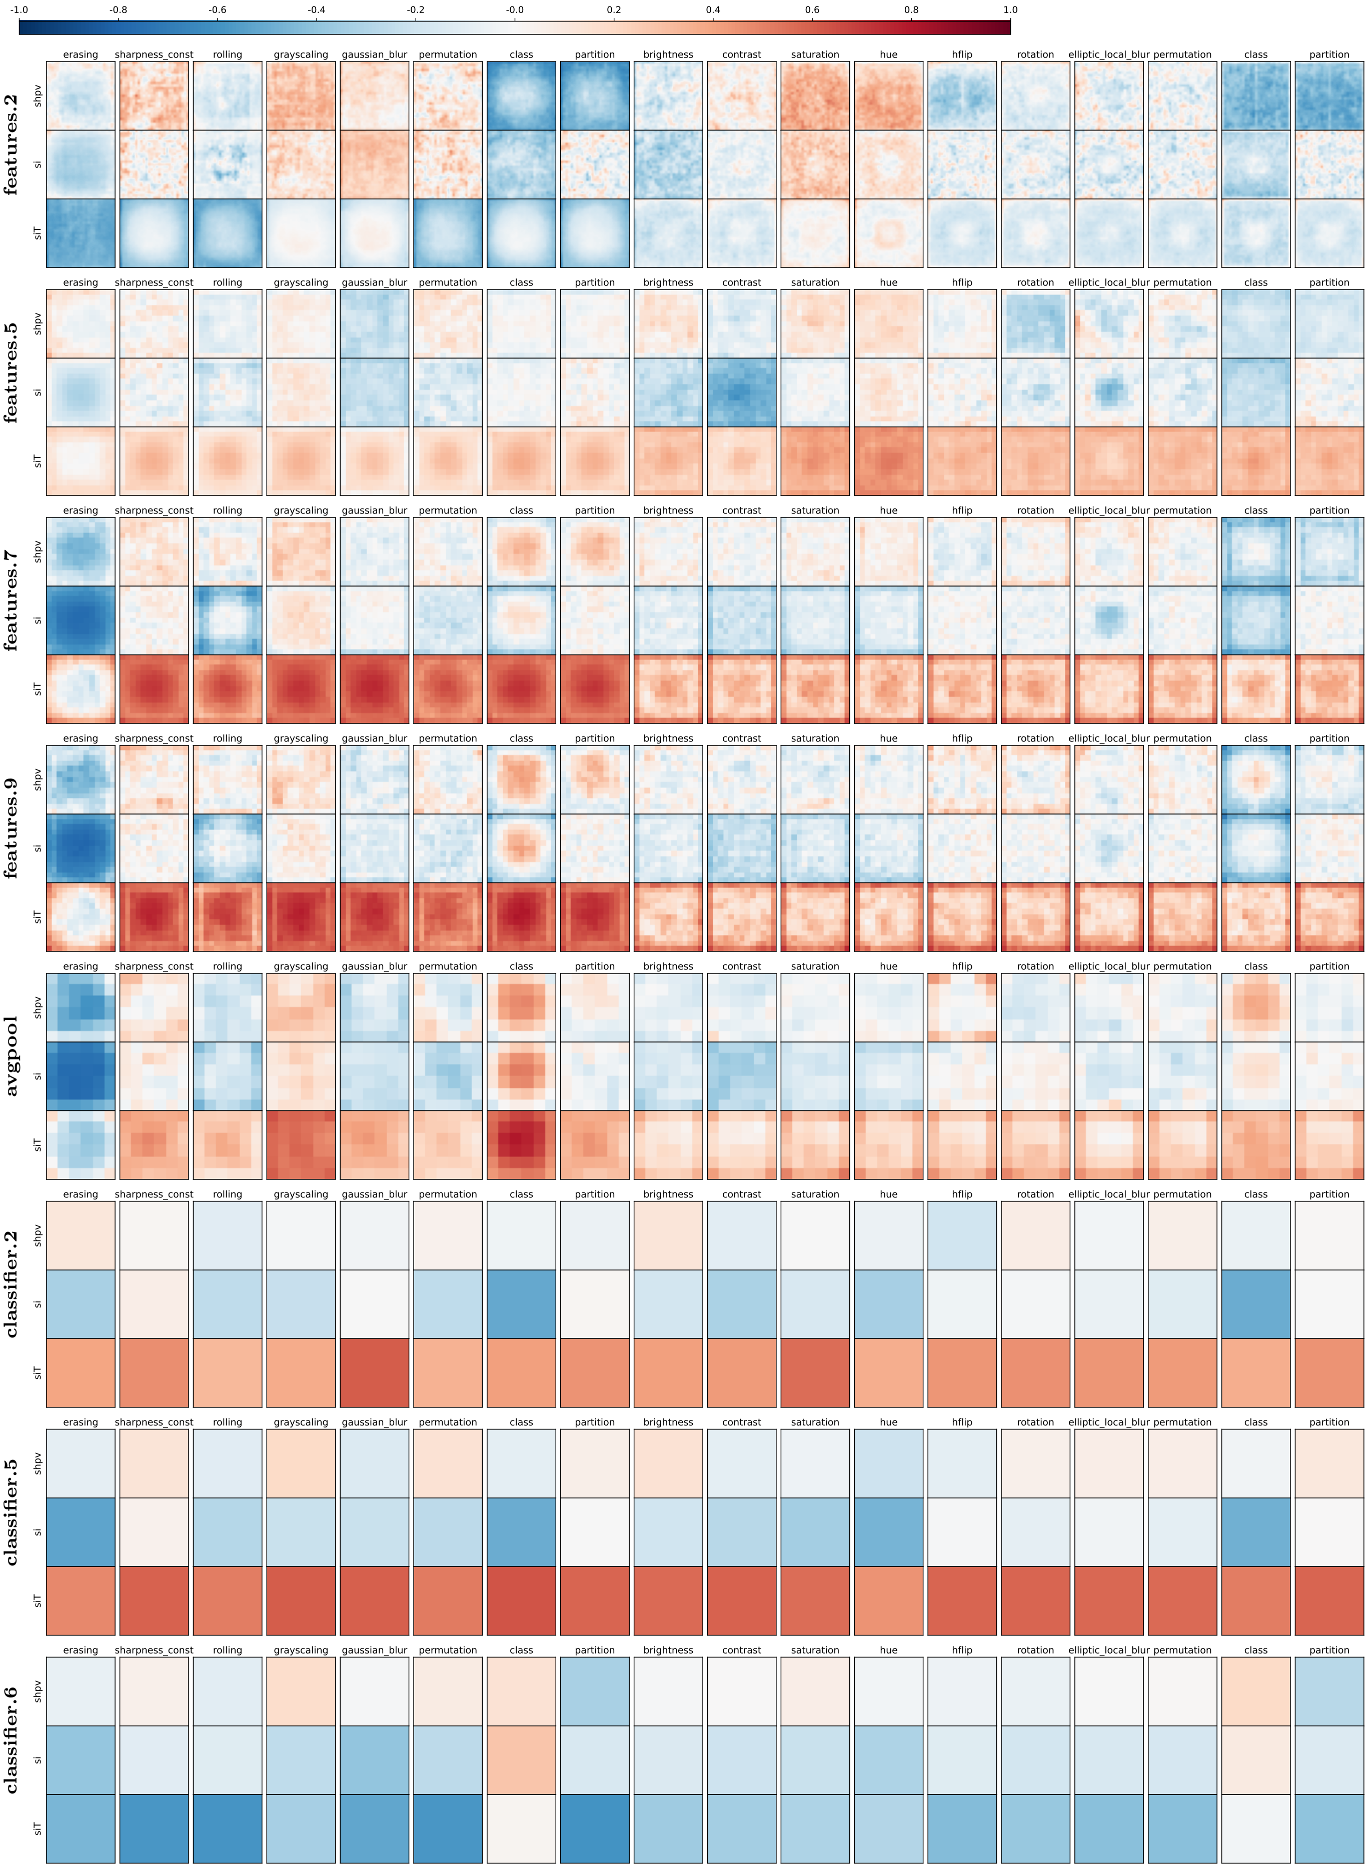


Figure S7.3 (b): Spatial maps for unit-wise correlations between sensitivities and coefficients of variation (AlexNet).

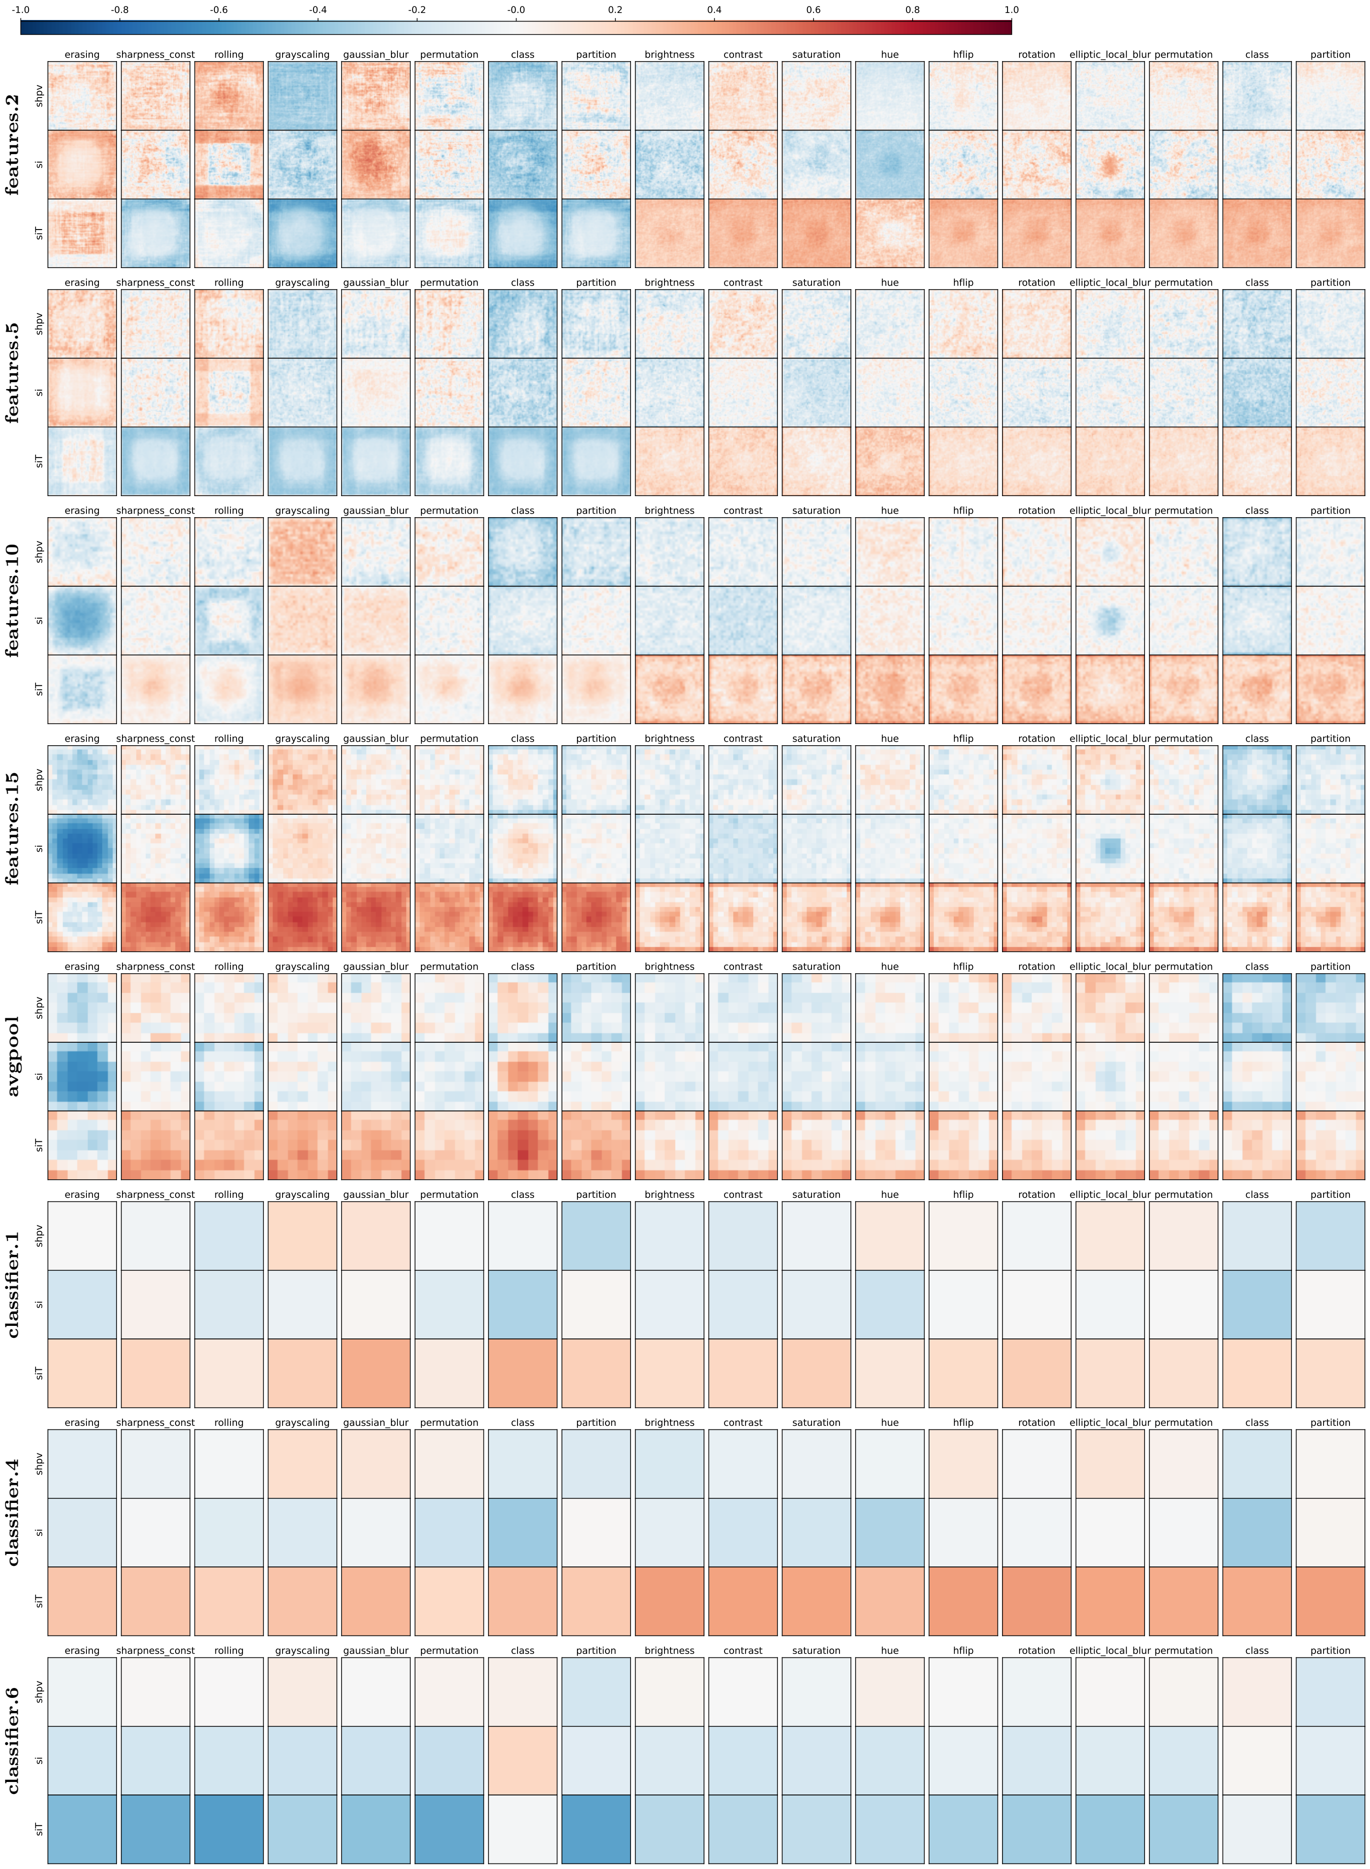


Figure S7.3 (c): Spatial maps for unit-wise correlations between sensitivities and coefficients of variation (VGG11).

# 4 Confusion matrices from Linear Discriminant Analysis (LDA) of the estimated sensitivities

Figures S7.4 (a)–S7.4 (c) are organized as follows. Each figure contains parts related to the network's convolutional checkpoints selected for sensitivity analysis in this study. The corresponding name of checkpoint is given on the left of a part. Each part is composed of two blocks, *augmentation set 1* and *augmentation set 2* respectively, divided into three column sub-blocks, corresponding to the Shapley values (*shpv*), the first-order Sobol indices (*si*), and the total Sobol indices (*siT*). The rows of a single confusion matrix encode the true SA variables, and the columns correspond to labels predicted by LDA.

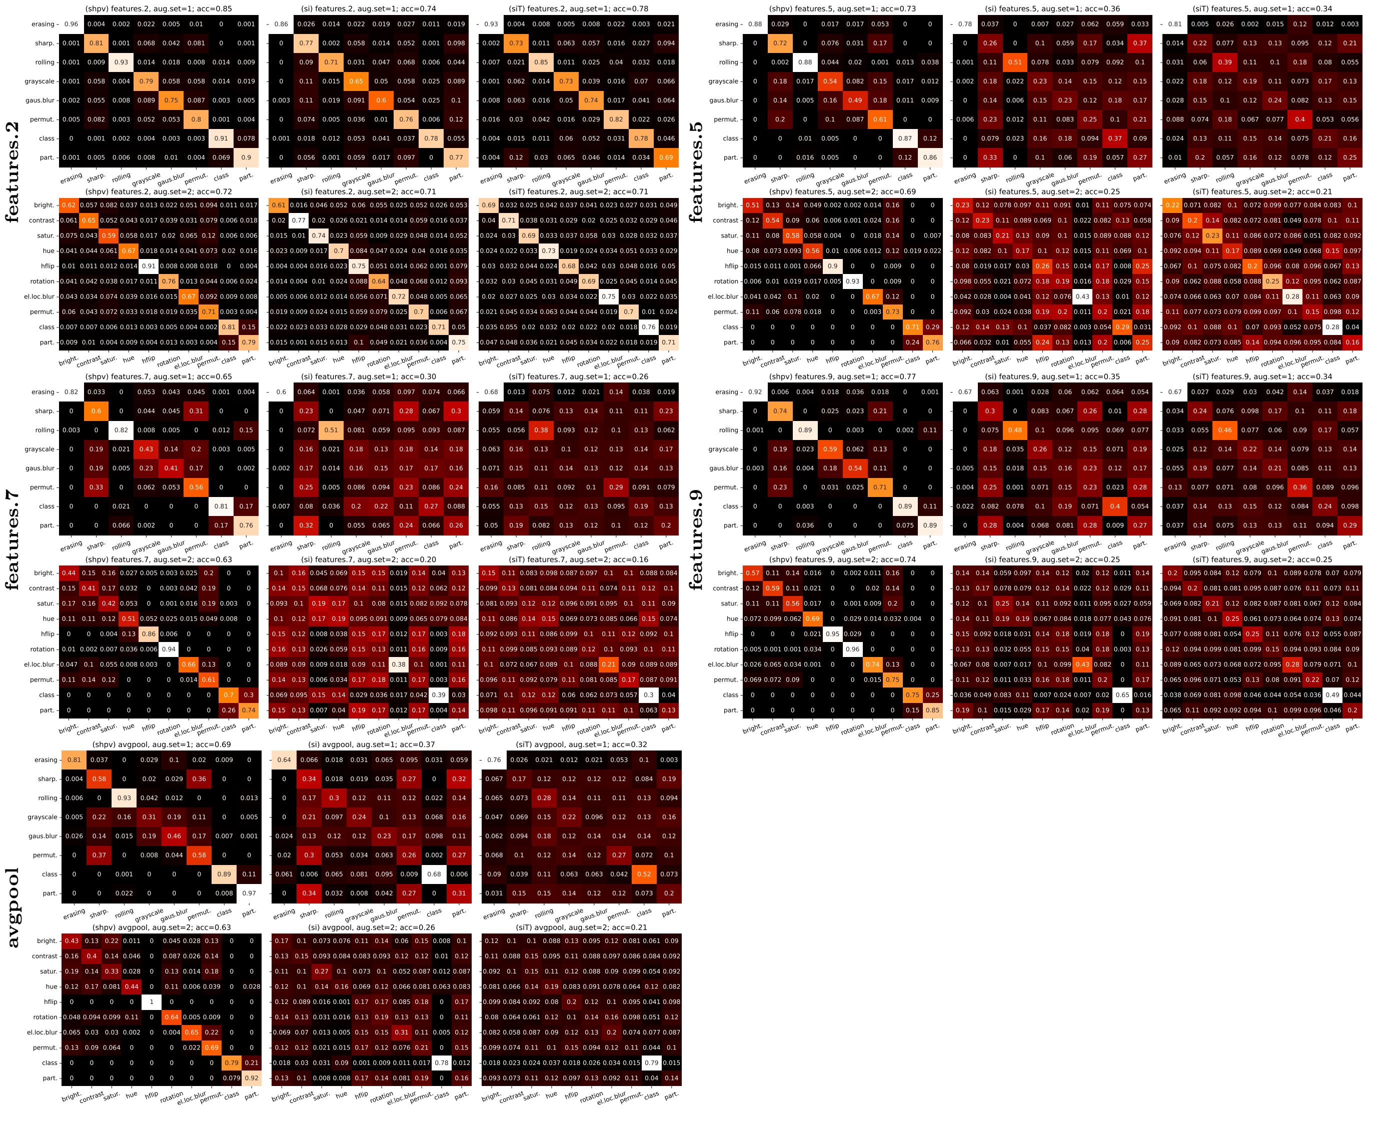


Figure S7.4 (a): Confusion matrix of LDA predictions of the SA variables for AlexNet.

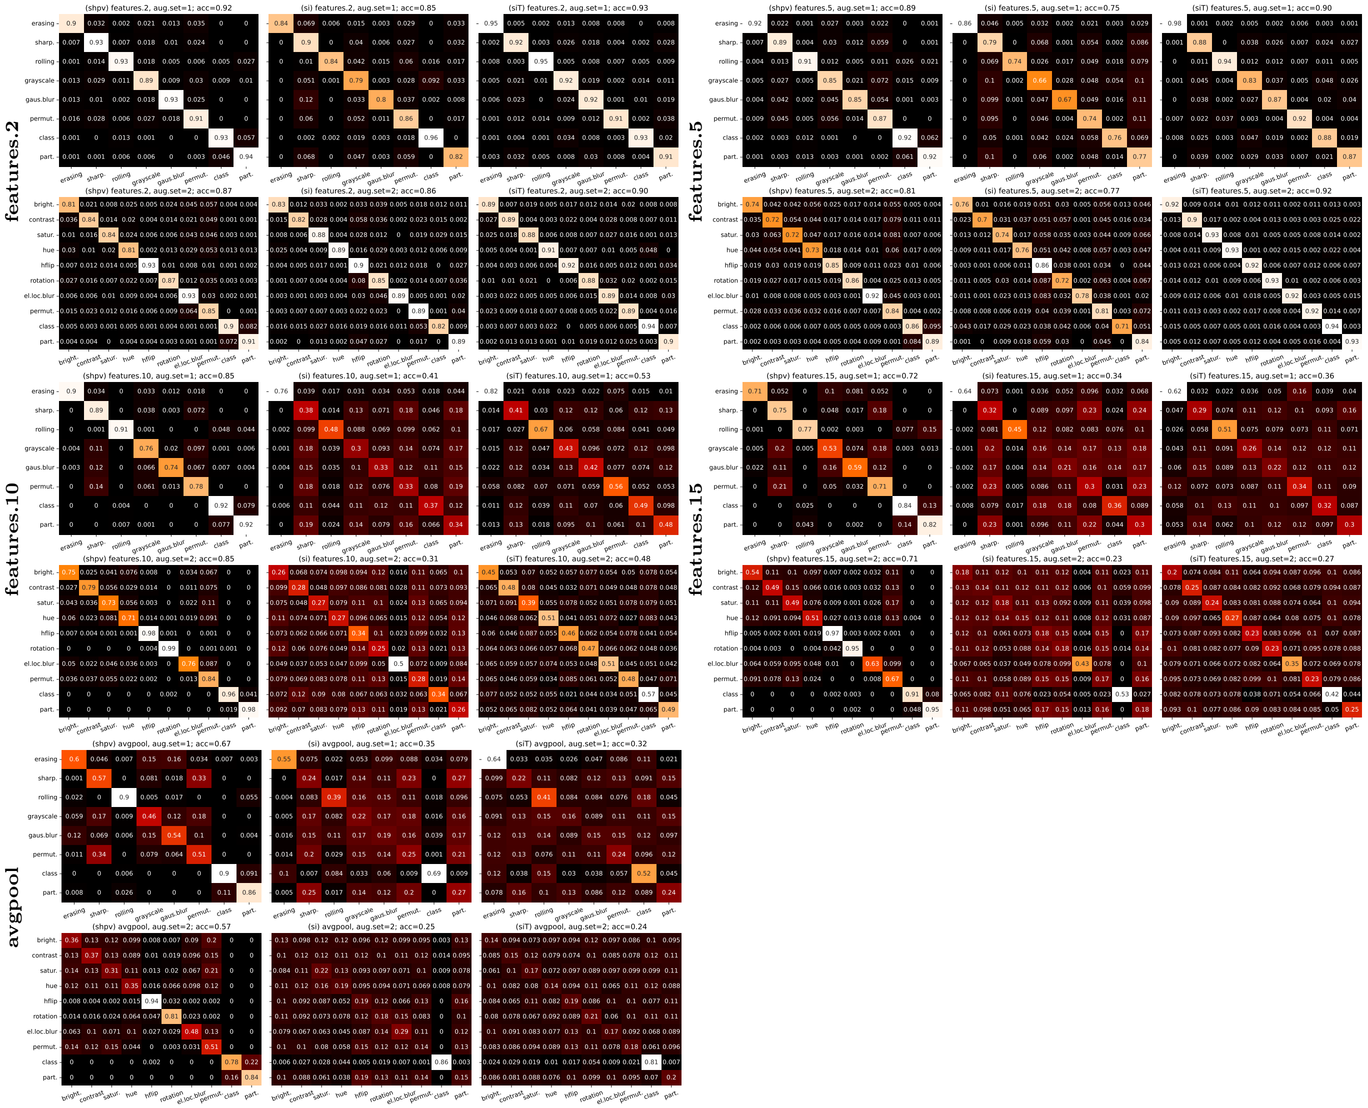

Figure S7.4 (b): Confusion matrix of LDA predictions of the SA variables for VGG11.

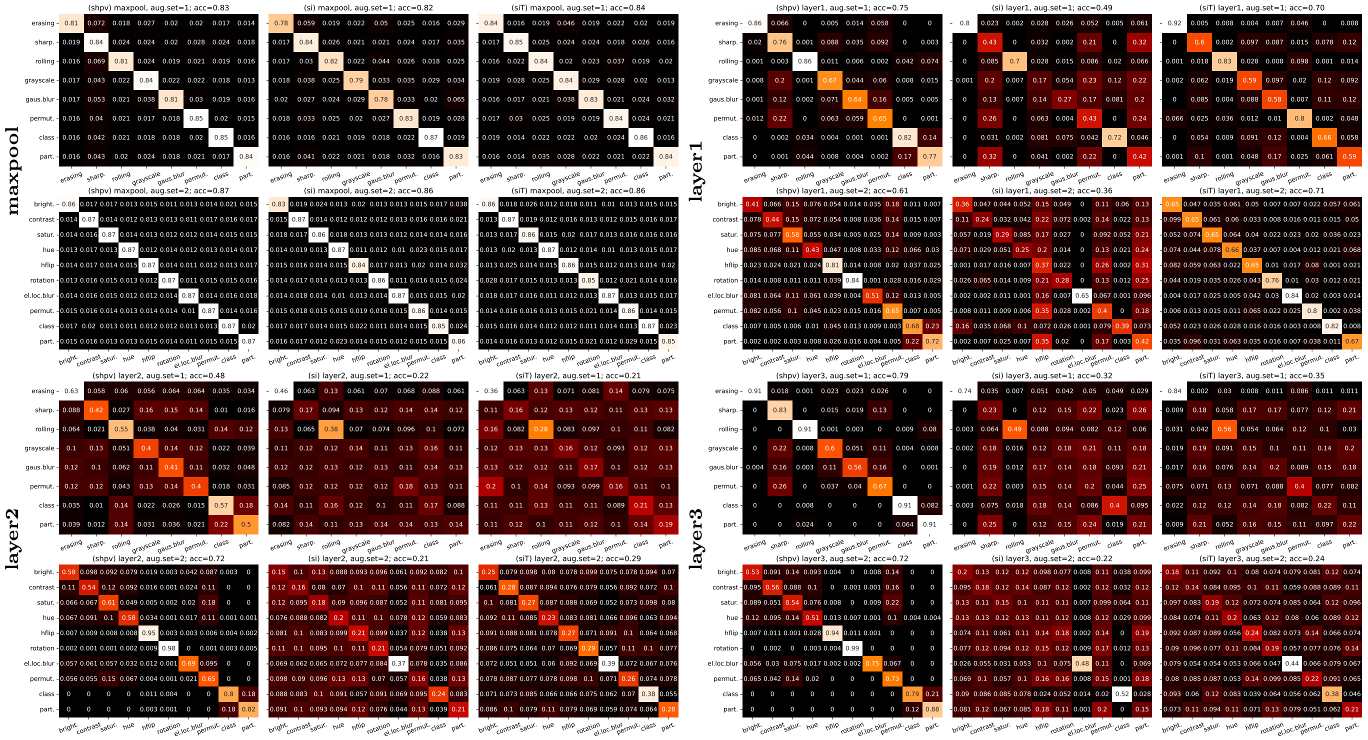

Figure S7.4 (c): Confusion matrix of LDA predictions of the SA variables for ResNet18.

# 5 Masked activations: hierarchical clustering analysis (HCA) of the prediction patterns

Figures S7.5 (a)–S7.5 (c) are formatted as follows. Cluster labels are given in the "*augmentation name – SA variable*" format, where the first entry is the name of augmentation used to transform the input to the network, and the second is a sensitivity analysis variable used for masking. The dashed lines correspond to the distance cut-off during the initial cluster assignment. A colour scheme was used to facilitate the distinguishing of neighbouring initial clusters. Each figure comprises two parts, *augmentation set 1* and *augmentation set 2* respectively, divided into three columns corresponding to the Shapley values (*shpv*), the first-order Sobol indices (*si*), and the total Sobol indices (*siT*).

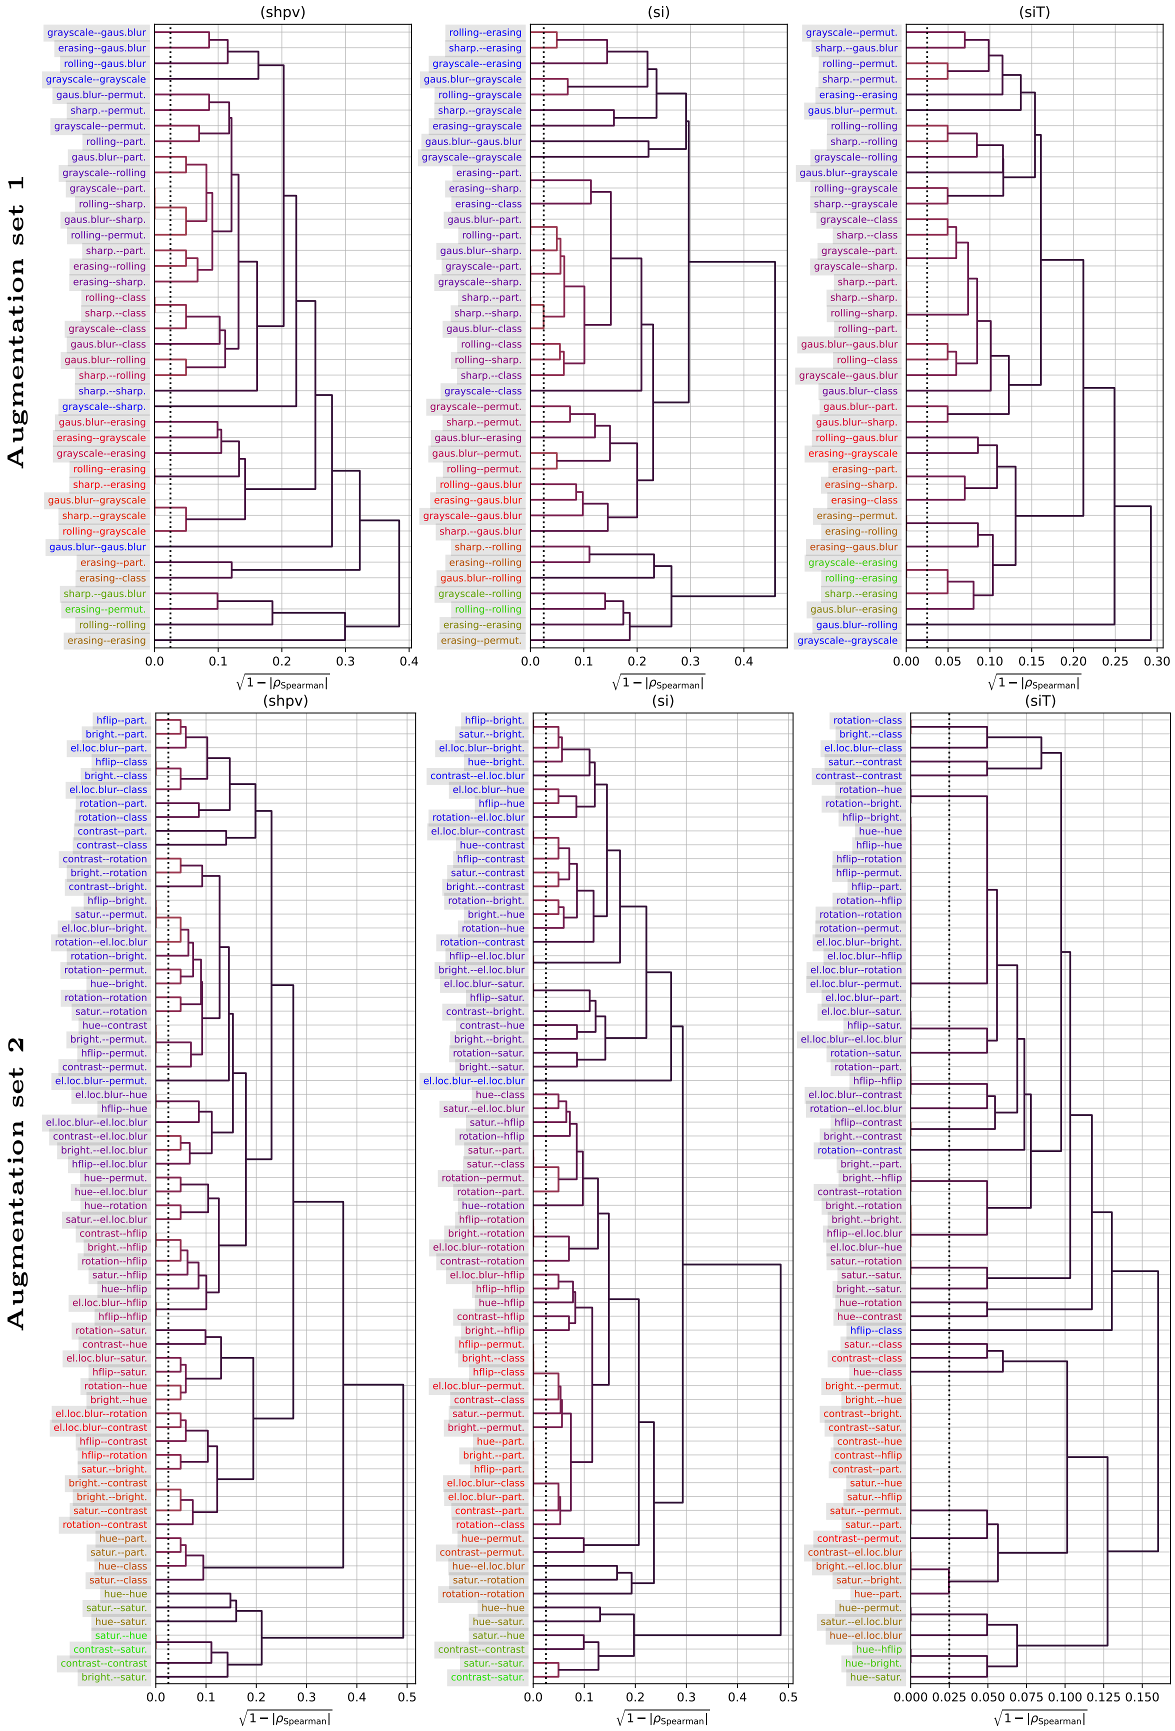


Figure S7.5 (a): HCA of the masked prediction patterns for AlexNet.

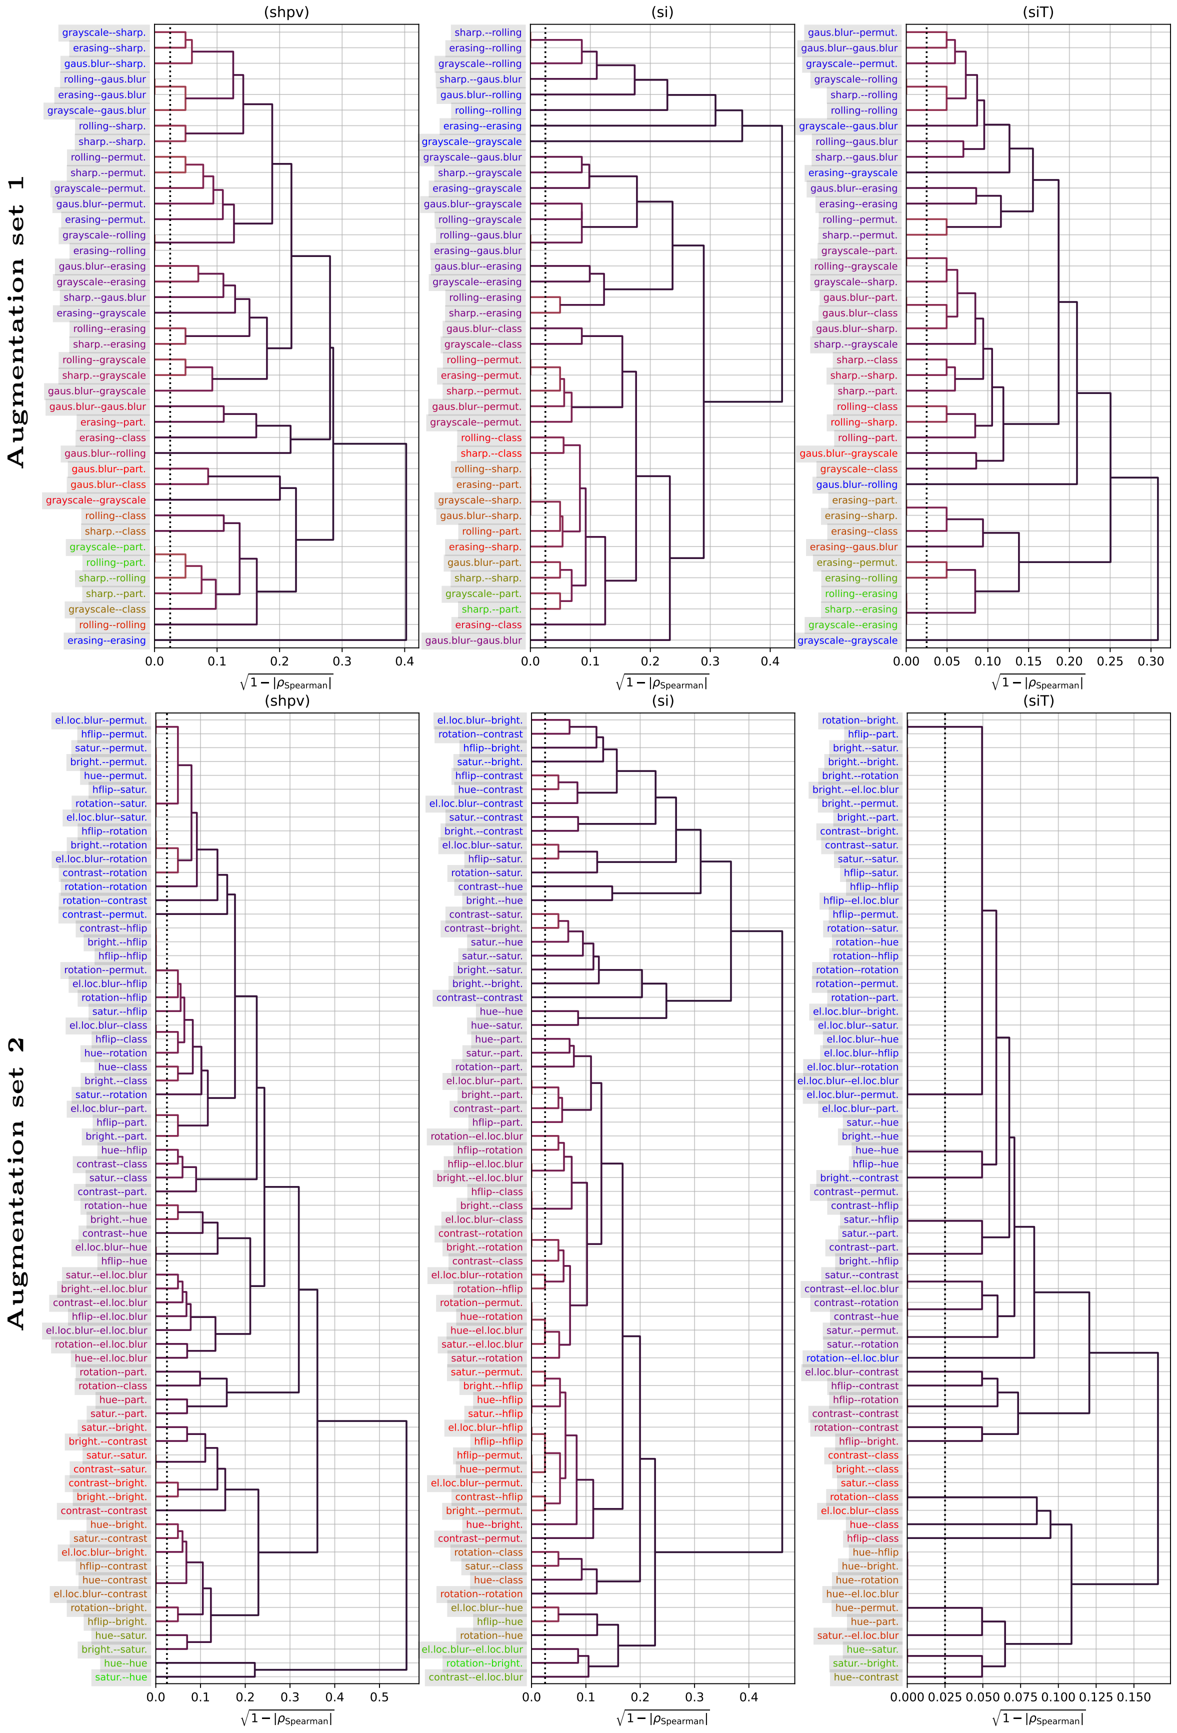


Figure S7.5 (b): HCA of the masked prediction patterns for VGG11.

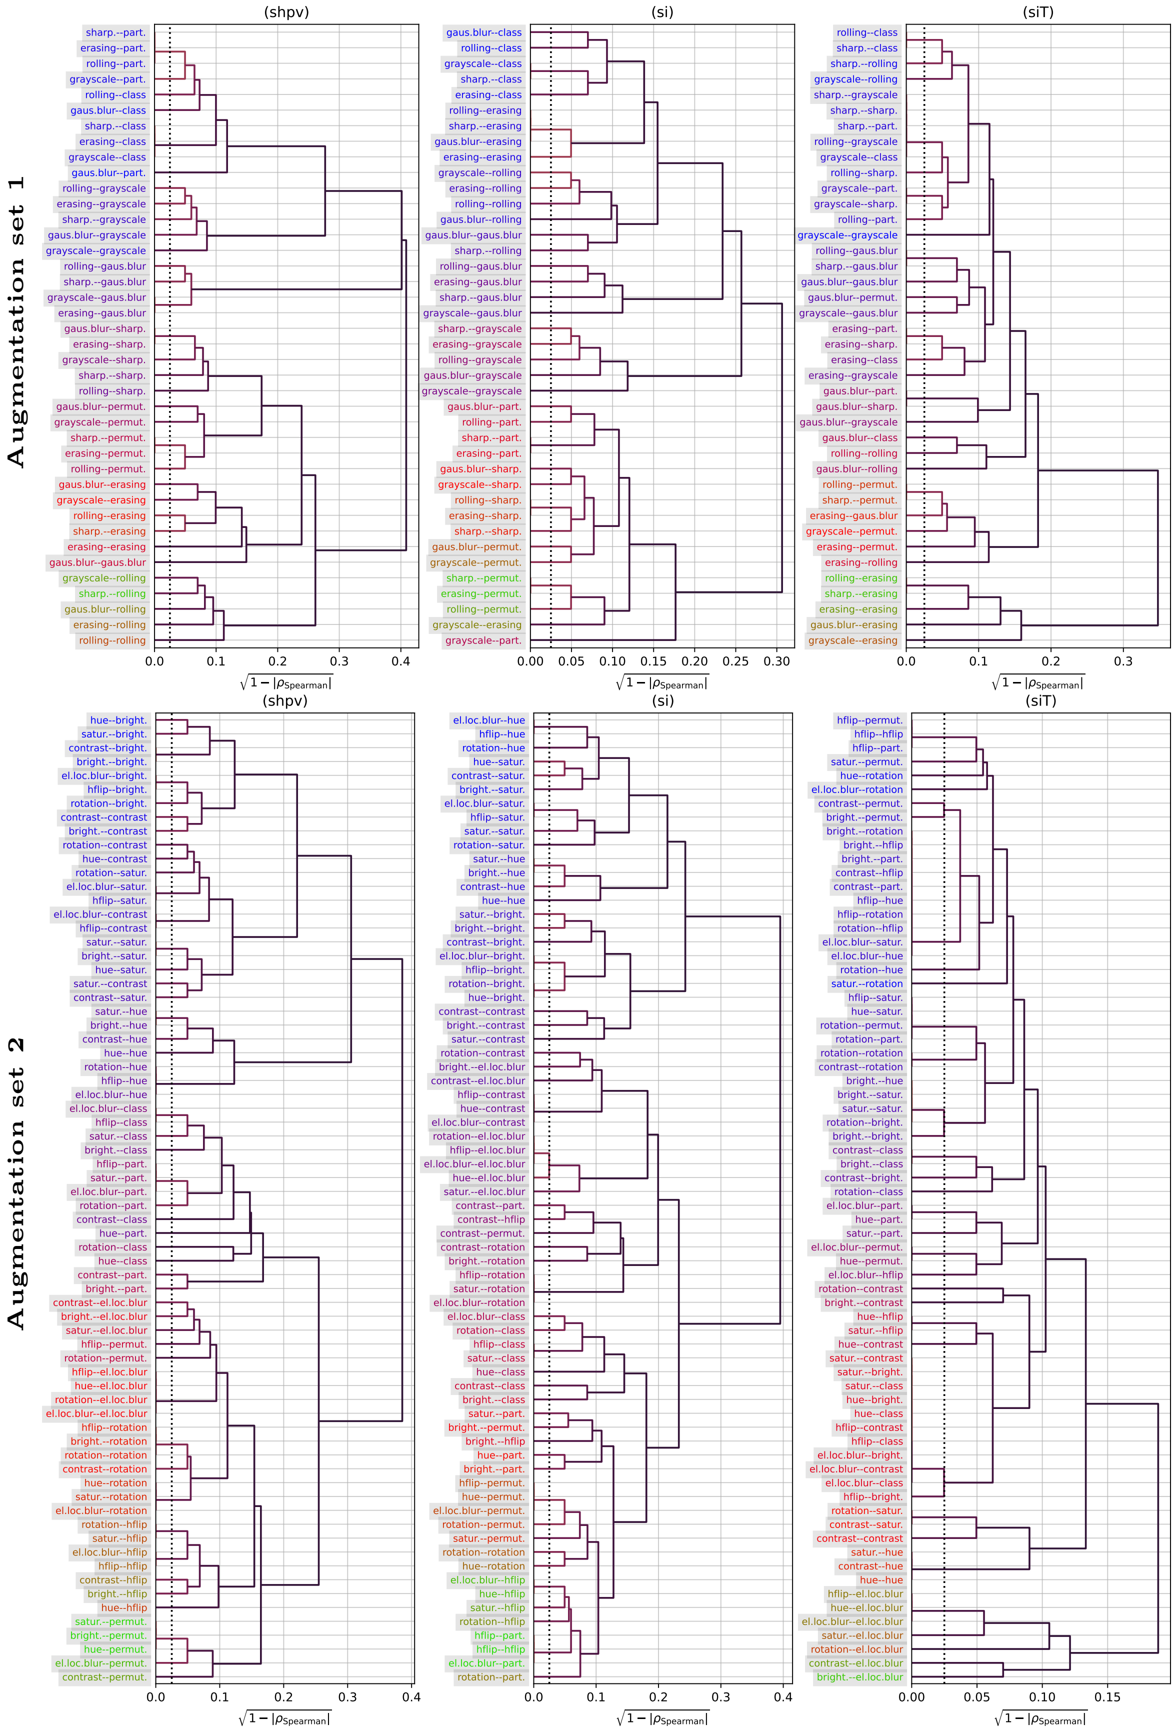


Figure S7.5 (c): HCA of the masked prediction patterns for ResNet18.

# 6 Single-class sensitivity analysis: relating single-class sensitivities and masked-activation predictions

In this section, we present the results demonstrating the deviation of the predictions when the activations related to the convolutional checkpoints are interfered with masks composed on the basis of the first-order Sobol indices and Shapley values. The networks' input was augmented using a single transform, and sensitivity analysis variables used for masking coincided with the corresponding augmentation of input. As previously, activations corresponding to the most sensitive values ($(1-q)\cdot 100\%$) were multiplied by the coefficient $\alpha$, $q \in \{0.5, 0.6, 0.7, 0.8, 0.9\}$, $\alpha \in \{0, 0.5, 1.5\}$ (Tables S7.6(a)–S7.6(b), S7.6(d)–S7.6(f)). One of the tables of this series is presented in the main text of the current work as Table 4. Besides, activations were multiplied by the sensitive values themselves, what we refer to as "raw mask", and by the inverted version of such mask (Table S7.6(c)), $m_{i,j}^{(\text{inv})} = 1 - m_{i,j}^{(\text{raw})}$, where $m_{i,j}^{(\text{inv})}, m_{i,j}^{(\text{raw})} \in [0,1]$ are $(i,j)$-th values of the inverted and raw masks, $(i,j)$ are row and column indices of the mask. The relation between single-class sensitivities and masked-activation predictions was estimated in terms of mean Jaccard indices between top-5 predictions and top-5 sensitive classes. All computations were made using the validation partition of the ILSVRC dataset.

Table S7.6(a): Mean Jaccard indices between top-5 masked predictions and top-5 sensitive classes extracted using Sobol indices computed for the final (classifying) layer. The sensitivity analysis variable used for masking (convolutional checkpoints only) is the same as the input augmentation. Activations corresponding to the $(1-q)\cdot 100\%$ top sensitivity values per checkpoint were multiplied by $\alpha = 0$.

| **Augmentation** | **AlexNet** | | | | | **VGG11** | | | | | **ResNet18** | | | | |
|---|---|---|---|---|---|---|---|---|---|---|---|---|---|---|---|
| **of input** | **q=0.5** | **q=0.6** | **q=0.7** | **q=0.8** | **q=0.9** | **q=0.5** | **q=0.6** | **q=0.7** | **q=0.8** | **q=0.9** | **q=0.5** | **q=0.6** | **q=0.7** | **q=0.8** | **q=0.9** |
| **Erasing** | .0 | .0 | .0 | .0001 | .0007 | .0023 | .002 | .0024 | .0029 | .0023 | .0 | .0 | .0 | .0001 | .0012 |
| **Sharp.** | .0 | .0003 | .001 | .0021 | .0026 | .0 | .012 | .0078 | .004 | .0037 | .0 | .0 | .0 | .0 | .0009 |
| **Rolling** | .0011 | .0017 | .0023 | .0029 | .0031 | .0062 | .0034 | .0026 | .0026 | .0034 | .0 | .0 | .0002 | .0007 | .0023 |
| **Grayscale** | .0 | .0003 | .0008 | .0016 | .0017 | .0058 | .0022 | .0017 | .0017 | .0021 | .0 | .0001 | .0004 | .0012 | .0019 |
| **Gaus.blur** | .0002 | .0003 | .0004 | .0007 | .0017 | .001 | .0033 | .0022 | .0018 | .0019 | .0 | .0 | .0006 | .0008 | .0008 |
| **Bright.** | .0006 | .0002 | .0002 | .0007 | .0021 | .008 | .0058 | .0047 | .0039 | .0036 | .0 | .0 | .0 | .0001 | .0027 |
| **Contrast.** | .0251 | .0245 | .0202 | .0109 | .0032 | .0106 | .0046 | .0026 | .0024 | .0024 | .0 | .0 | .0027 | .0048 | .0018 |
| **Satur.** | .0 | .0 | .0016 | .0028 | .0023 | .0613 | .0128 | .0046 | .0035 | .0034 | .0 | .0 | .0001 | .0014 | .0017 |
| **Hue** | .0008 | .0007 | .0022 | .0024 | .0031 | .0222 | .0068 | .004 | .0031 | .0032 | .0 | .0004 | .0014 | .0025 | .0027 |
| **Hflip** | .0 | .0033 | .0079 | .0057 | .0041 | .1111 | .0206 | .0123 | .0064 | .0039 | .0 | .0 | .0 | .0011 | .0019 |
| **Rotation** | .0 | .0001 | .0005 | .0019 | .0032 | .0017 | .0022 | .0032 | .0035 | .0034 | .0065 | .0037 | .0002 | .0004 | .0023 |
| **El.loc.blur** | .0163 | .0094 | .0071 | .0033 | .0022 | .023 | .0121 | .0055 | .0031 | .0028 | .0 | .0 | .0001 | .0051 | .0054 |

Table S7.6(b): Mean Jaccard indices between top-5 masked predictions and top-5 sensitive classes extracted using Sobol indices computed for the final (classifying) layer. The sensitivity analysis variable used for masking (convolutional checkpoints only) is the same as the input augmentation. Activations corresponding to the $(1-q)\cdot 100\%$ top sensitivity values per checkpoint were multiplied by $\alpha = 0.5$.

| **Augmentation** | **AlexNet** | | | | | **VGG11** | | | | | **ResNet18** | | | | |
|---|---|---|---|---|---|---|---|---|---|---|---|---|---|---|---|
| **of input** | **q=0.5** | **q=0.6** | **q=0.7** | **q=0.8** | **q=0.9** | **q=0.5** | **q=0.6** | **q=0.7** | **q=0.8** | **q=0.9** | **q=0.5** | **q=0.6** | **q=0.7** | **q=0.8** | **q=0.9** |
| **Erasing** | .0003 | .0003 | .0005 | .0008 | .0018 | .0028 | .0027 | .0027 | .0025 | .0023 | .0001 | .0002 | .0007 | .0021 | .0029 |
| **Sharp.** | .0023 | .0022 | .0025 | .0027 | .0028 | .009 | .0037 | .0036 | .0036 | .0037 | .0002 | .0011 | .0016 | .002 | .0023 |
| **Rolling** | .003 | .0029 | .0029 | .0031 | .0033 | .004 | .0035 | .0033 | .0032 | .0031 | .0015 | .0018 | .0026 | .0041 | .003 |
| **Grayscale** | .0021 | .0021 | .0022 | .0022 | .0023 | .0023 | .0021 | .002 | .002 | .0023 | .0028 | .0016 | .0014 | .0017 | .0022 |
| **Gaus.blur** | .003 | .0024 | .0023 | .0022 | .0018 | .0015 | .0016 | .0015 | .0016 | .0018 | .0009 | .0013 | .0018 | .0023 | .0019 |
| **Bright.** | .0017 | .0015 | .0016 | .0018 | .0021 | .0039 | .0038 | .0036 | .0035 | .0035 | .0007 | .0012 | .002 | .002 | .0028 |
| **Contrast.** | .0034 | .0039 | .0042 | .0038 | .0029 | .0026 | .0023 | .0023 | .0023 | .0024 | .0051 | .0064 | .0067 | .0042 | .0022 |
| **Satur.** | .0018 | .0019 | .0022 | .0026 | .0027 | .0038 | .0033 | .0032 | .0033 | .0039 | .0016 | .0028 | .0043 | .0028 | .0023 |
| **Hue** | .0049 | .0041 | .0037 | .0034 | .0031 | .004 | .0033 | .003 | .0028 | .0026 | .0032 | .0019 | .0019 | .0022 | .0023 |
| **Hflip** | .0027 | .004 | .0041 | .0037 | .0036 | .0059 | .0042 | .0038 | .0033 | .003 | .0 | .0011 | .0015 | .0022 | .0025 |
| **Rotation** | .0031 | .0031 | .0031 | .0033 | .0034 | .0035 | .0034 | .0033 | .0033 | .0032 | .0023 | .0029 | .0033 | .004 | .0036 |
| **El.loc.blur** | .0029 | .0024 | .0025 | .0023 | .0022 | .0035 | .003 | .0027 | .0026 | .0026 | .004 | .0038 | .0054 | .0063 | .0043 |

Table S7.6(c): Mean Jaccard indices between top-5 masked predictions and top-5 sensitive classes extracted using sensitivity values computed for the final (classifying) layer. The sensitivity analysis variable used for masking (convolutional checkpoints only) is the same as the input augmentation. Activations were multiplied either by a mask ("raw") or its complement ("inv.").

| **Augmentation of input** | **Shapley values** | | | | | | **Sobol indices** | | | | | |
|---|---|---|---|---|---|---|---|---|---|---|---|---|
| | **AlexNet** | | **VGG11** | | **ResNet18** | | **AlexNet** | | **VGG11** | | **ResNet18** | |
| | **raw** | **inv.** | **raw** | **inv.** | **raw** | **inv.** | **raw** | **inv.** | **raw** | **inv.** | **raw** | **inv.** |
| **Erasing** | .0 | .0022 | .0 | .003 | .0 | .0025 | .0 | .0047 | .0 | .0023 | .0 | .0065 |
| **Sharp.** | .0 | .0035 | .0 | .0026 | .0 | .0023 | .0 | .0028 | .0 | .0037 | .0 | .0023 |
| **Rolling** | .0 | .0031 | .0 | .0026 | .0 | .0026 | .0 | .003 | .0 | .0029 | .0 | .0027 |
| **Grayscale** | .0 | .0005 | .0 | .0013 | .0 | .002 | .0 | .0023 | .0 | .0024 | .0 | .0027 |
| **Gaus.blur** | .0 | .003 | .0 | .0026 | .0 | .0029 | .0 | .0023 | .0 | .0019 | .0 | .0022 |
| **Bright.** | .0001 | .002 | .0 | .0035 | .0 | .0032 | .0 | .002 | .0 | .0028 | .0 | .0027 |
| **Contrast.** | .0 | .0035 | .0 | .002 | .0 | .0031 | .0 | .0028 | .1111 | .0026 | .0 | .0046 |
| **Satur.** | .0 | .0025 | .0 | .0026 | .0 | .0025 | .0 | .0035 | .0 | .0049 | .0 | .0026 |
| **Hue** | .0 | .0018 | .0 | .0023 | .0 | .0015 | .0 | .0038 | .0 | .0019 | .0 | .0036 |
| **Hflip** | .0 | .0024 | .0 | .0025 | .0 | .0027 | .0 | .0035 | .0 | .0028 | .0 | .0028 |
| **Rotation** | .0 | .0026 | .0461 | .0021 | .0 | .0028 | .0 | .0032 | .0 | .0032 | .0 | .0032 |
| **El.loc.blur** | .0 | .0025 | .0 | .0029 | .0 | .0026 | .0 | .0024 | .0 | .0024 | .0 | .0029 |

Table S7.6(d): Mean Jaccard indices between top-5 masked predictions and top-5 sensitive classes extracted using Shapley values computed for the final (classifying) layer. The sensitivity analysis variable used for masking (convolutional checkpoints only) is the same as the input augmentation. Activations corresponding to the $(1-q)\cdot 100\%$ top sensitivity values per checkpoint were multiplied by $\alpha = 0$.

| **Augmentation of input** | **AlexNet** | | | | | **VGG11** | | | | | **ResNet18** | | | | |
|---|---|---|---|---|---|---|---|---|---|---|---|---|---|---|---|
| | **q=0.5** | **q=0.6** | **q=0.7** | **q=0.8** | **q=0.9** | **q=0.5** | **q=0.6** | **q=0.7** | **q=0.8** | **q=0.9** | **q=0.5** | **q=0.6** | **q=0.7** | **q=0.8** | **q=0.9** |
| **Erasing** | .0268 | .0207 | .0165 | .0098 | .0043 | .0022 | .003 | .0037 | .0036 | .0038 | .0004 | .0003 | .0002 | .0004 | .0013 |
| **Sharp.** | .0032 | .0081 | .0074 | .0044 | .0032 | .0 | .0001 | .0005 | .0014 | .0028 | .0 | .0 | .0 | .0039 | .0034 |
| **Rolling** | .0 | .0 | .0001 | .0006 | .0024 | .0 | .0 | .0001 | .0013 | .0026 | .0 | .0002 | .0006 | .0013 | .0019 |
| **Grayscale** | .0 | .0 | .0001 | .0002 | .0002 | .0 | .0 | .0001 | .0003 | .0007 | .0 | .0 | .0002 | .0024 | .0035 |
| **Gaus.blur** | .0026 | .0032 | .0027 | .0026 | .0036 | .0 | .0001 | .001 | .0021 | .0025 | .0 | .0 | .0 | .0002 | .0024 |
| **Bright.** | .0001 | .0003 | .0015 | .002 | .0018 | .0 | .0001 | .0007 | .002 | .003 | .0162 | .0001 | .0001 | .0025 | .0039 |
| **Contrast.** | .0815 | .0476 | .0136 | .0041 | .0027 | .0392 | .0231 | .0096 | .0051 | .0035 | .0 | .0 | .0 | .0002 | .0021 |
| **Satur.** | .0303 | .0185 | .0057 | .0049 | .0054 | .0002 | .0003 | .0015 | .0021 | .0023 | .0 | .0001 | .0001 | .0022 | .0028 |
| **Hue** | .0 | .0001 | .0008 | .0017 | .0016 | .0041 | .005 | .0043 | .0035 | .0031 | .0 | .0 | .0012 | .0016 | .0017 |
| **Hflip** | .0 | .0 | .0 | .0002 | .0014 | .0 | .0 | .0001 | .0008 | .0022 | .0 | .0 | .0001 | .0013 | .0033 |
| **Rotation** | .0001 | .0003 | .0005 | .0015 | .0025 | .0009 | .0011 | .0015 | .0023 | .002 | .0 | .0001 | .001 | .0022 | .002 |
| **El.loc.blur** | .0 | .0 | .0003 | .0013 | .0021 | .0 | .0 | .0015 | .0025 | .0029 | .0 | .0 | .0001 | .0001 | .0007 |

Table S7.6(e): Mean Jaccard indices between top-5 masked predictions and top-5 sensitive classes extracted using Shapley values computed for the final (classifying) layer. The sensitivity analysis variable used for masking (convolutional checkpoints only) is the same as the input augmentation. Activations corresponding to the $(1-q)\cdot 100\%$ top sensitivity values per checkpoint were multiplied by $\alpha = 0.5$.

| **Augmentation** | **AlexNet** | | | | | **VGG11** | | | | | **ResNet18** | | | | |
|---|---|---|---|---|---|---|---|---|---|---|---|---|---|---|---|
| **of input** | **q=0.5** | **q=0.6** | **q=0.7** | **q=0.8** | **q=0.9** | **q=0.5** | **q=0.6** | **q=0.7** | **q=0.8** | **q=0.9** | **q=0.5** | **q=0.6** | **q=0.7** | **q=0.8** | **q=0.9** |
| **Erasing** | .0035 | .0032 | .003 | .0028 | .0024 | .0028 | .0033 | .0035 | .0036 | .0032 | .002 | .002 | .0019 | .0019 | .0021 |
| **Sharp.** | .004 | .0036 | .0035 | .0035 | .0034 | .0013 | .0026 | .0027 | .0028 | .0027 | .0007 | .0002 | .0008 | .0017 | .002 |
| **Rolling** | .0013 | .0017 | .0022 | .0027 | .0026 | .0016 | .0021 | .0024 | .0025 | .0026 | .0002 | .0004 | .0012 | .0018 | .0021 |
| **Grayscale** | .0002 | .0004 | .0004 | .0004 | .0004 | .0008 | .0008 | .0009 | .001 | .0012 | .0002 | .0007 | .0015 | .0019 | .0023 |
| **Gaus.blur** | .0026 | .0027 | .0029 | .003 | .0033 | .0015 | .0017 | .002 | .0023 | .0026 | .0008 | .0015 | .0024 | .0024 | .0025 |
| **Bright.** | .0022 | .0021 | .002 | .0019 | .0018 | .002 | .0025 | .0029 | .0032 | .0034 | .003 | .0027 | .0031 | .0038 | .0036 |
| **Contrast.** | .0045 | .0036 | .0031 | .003 | .0036 | .0041 | .0034 | .0028 | .0026 | .0024 | .0002 | .0002 | .0007 | .0018 | .0028 |
| **Satur.** | .0072 | .0053 | .0041 | .0039 | .0034 | .0024 | .0024 | .0025 | .0025 | .0025 | .0005 | .0009 | .0025 | .0037 | .0027 |
| **Hue** | .0017 | .0026 | .0023 | .0021 | .002 | .0027 | .0028 | .0029 | .0027 | .0025 | .0005 | .0016 | .0019 | .0021 | .002 |
| **Hflip** | .0016 | .0016 | .0018 | .0022 | .0023 | .0013 | .0016 | .0021 | .0023 | .0025 | .0011 | .0026 | .0034 | .0035 | .0032 |
| **Rotation** | .0011 | .0015 | .0019 | .0023 | .0027 | .0036 | .003 | .0024 | .0021 | .002 | .0006 | .0016 | .0021 | .002 | .0022 |
| **El.loc.blur** | .0019 | .0021 | .0023 | .0023 | .0023 | .0036 | .0035 | .0029 | .003 | .0029 | .0001 | .0002 | .0005 | .0009 | .0022 |

Table S7.6(f): Mean Jaccard indices between top-5 masked predictions and top-5 sensitive classes extracted using Shapley values computed for the final (classifying) layer. The sensitivity analysis variable used for masking (convolutional checkpoints only) is the same as the input augmentation. Activations corresponding to the $(1-q)\cdot 100\%$ top sensitivity values per checkpoint were multiplied by $\alpha = 1.5$.

| **Augmentation** | **AlexNet** | | | | | **VGG11** | | | | | **ResNet18** | | | | |
|---|---|---|---|---|---|---|---|---|---|---|---|---|---|---|---|
| **of input** | **q=0.5** | **q=0.6** | **q=0.7** | **q=0.8** | **q=0.9** | **q=0.5** | **q=0.6** | **q=0.7** | **q=0.8** | **q=0.9** | **q=0.5** | **q=0.6** | **q=0.7** | **q=0.8** | **q=0.9** |
| **Erasing** | .0004 | .0003 | .0002 | .0003 | .0005 | .0011 | .001 | .0009 | .001 | .0015 | .0002 | .0003 | .0007 | .0013 | .0023 |
| **Sharp.** | .0029 | .0035 | .0037 | .0037 | .0035 | .0012 | .0022 | .0024 | .0025 | .0026 | .0 | .0001 | .0003 | .0007 | .0014 |
| **Rolling** | .0011 | .0012 | .0011 | .0011 | .0014 | .0018 | .0019 | .002 | .0021 | .0023 | .0014 | .002 | .0017 | .0013 | .0014 |
| **Grayscale** | .001 | .0012 | .0013 | .0016 | .0012 | .0015 | .0018 | .0018 | .0016 | .0013 | .0 | .0007 | .0069 | .009 | .0022 |
| **Gaus.blur** | .0016 | .0018 | .0018 | .0019 | .0018 | .0027 | .0029 | .003 | .003 | .0029 | .0033 | .0041 | .0039 | .0026 | .0016 |
| **Bright.** | .0015 | .0018 | .0021 | .0024 | .0026 | .0032 | .0037 | .0043 | .0045 | .0044 | .049 | .0567 | .0691 | .0714 | .0678 |
| **Contrast.** | .0066 | .0048 | .0038 | .0032 | .0032 | .0015 | .0017 | .0019 | .002 | .0021 | .0001 | .0001 | .0003 | .001 | .002 |
| **Satur.** | .0008 | .0008 | .0008 | .0009 | .0012 | .0027 | .003 | .0031 | .0032 | .0032 | .0001 | .0003 | .0006 | .0008 | .0011 |
| **Hue** | .0005 | .0007 | .0008 | .0009 | .0008 | .0019 | .0017 | .0015 | .0013 | .0013 | .0001 | .0002 | .0003 | .0002 | .0003 |
| **Hflip** | .0026 | .0028 | .0028 | .0027 | .0025 | .0024 | .0027 | .0027 | .0028 | .0027 | .0007 | .0011 | .0017 | .0025 | .0029 |
| **Rotation** | .0034 | .0037 | .0037 | .0034 | .003 | .002 | .0019 | .0018 | .0017 | .0018 | .0055 | .0066 | .0058 | .0066 | .0041 |
| **El.loc.blur** | .0019 | .0021 | .0023 | .0025 | .0027 | .0015 | .0021 | .0024 | .0026 | .0027 | .0001 | .0001 | .0003 | .0007 | .0014 |

# 7 Correlation matrices between sensitivity variables

Figures S7.7 (a)–S7.7 (d) are arranged in the following way. Each figure consists of several parts related to the network's checkpoints selected for sensitivity analysis in this study. The corresponding name of a checkpoint is given on the left of a part. Each part comprises four blocks related to the input to the first layer with all channels (*original*) and its version separated into HSV channels and repeated respective times passed to the corresponding cropped subnetwork (*hue*, *saturation*, *value*). These blocks are divided into three column sub-blocks: Shapley values (*shpv*), the first-order Sobol indices (*si*), and the total Sobol indices (*siT*). Only lower triangular parts of the correlation matrices are displayed.

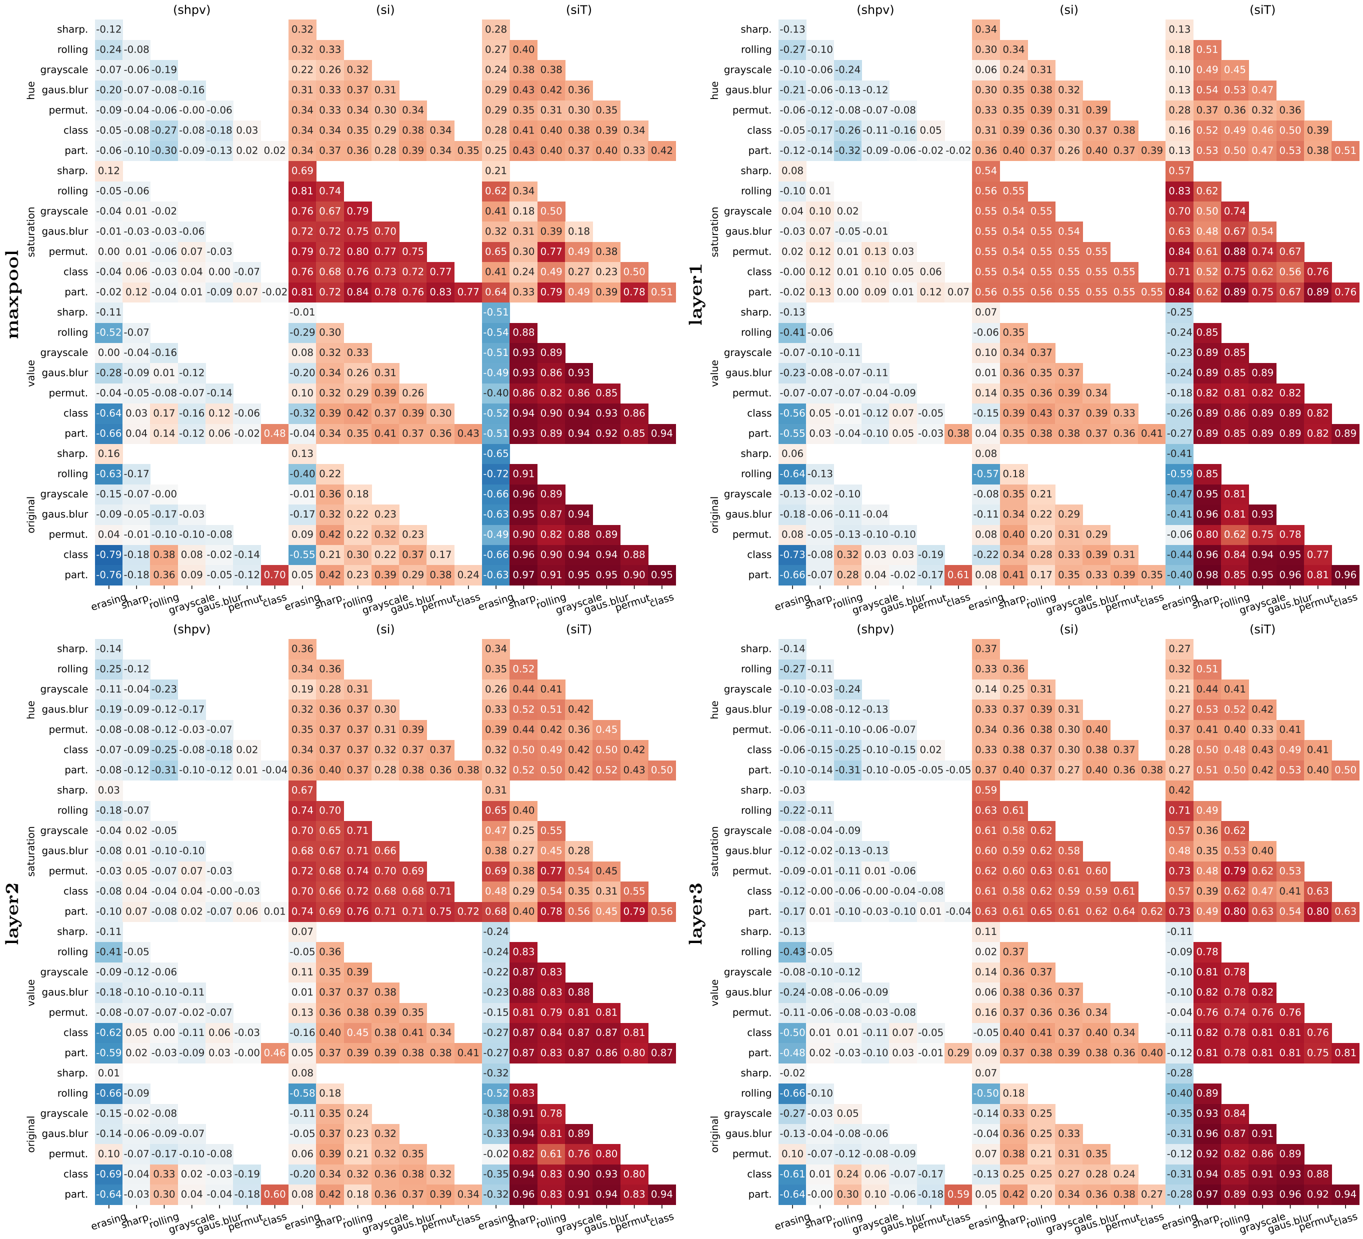


Figure S7.7 (a): Correlation matrices between sensitivity variables for ResNet18 (augmentation set 1).

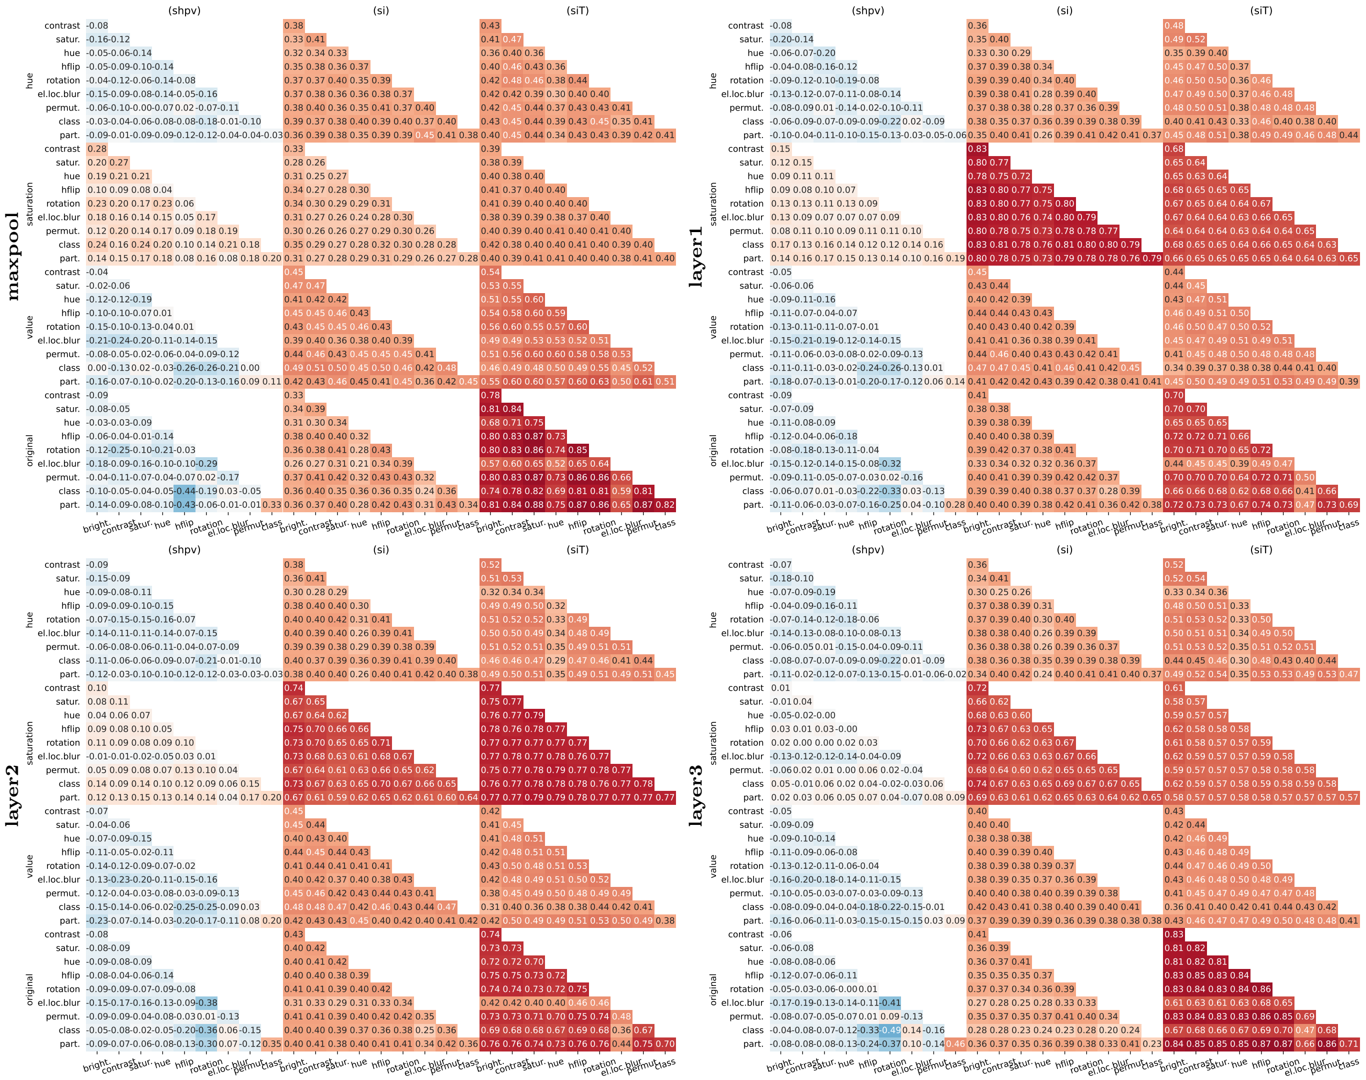


Figure S7.7 (b): Correlation matrices between sensitivity variables for ResNet18 (augmentation set 2).

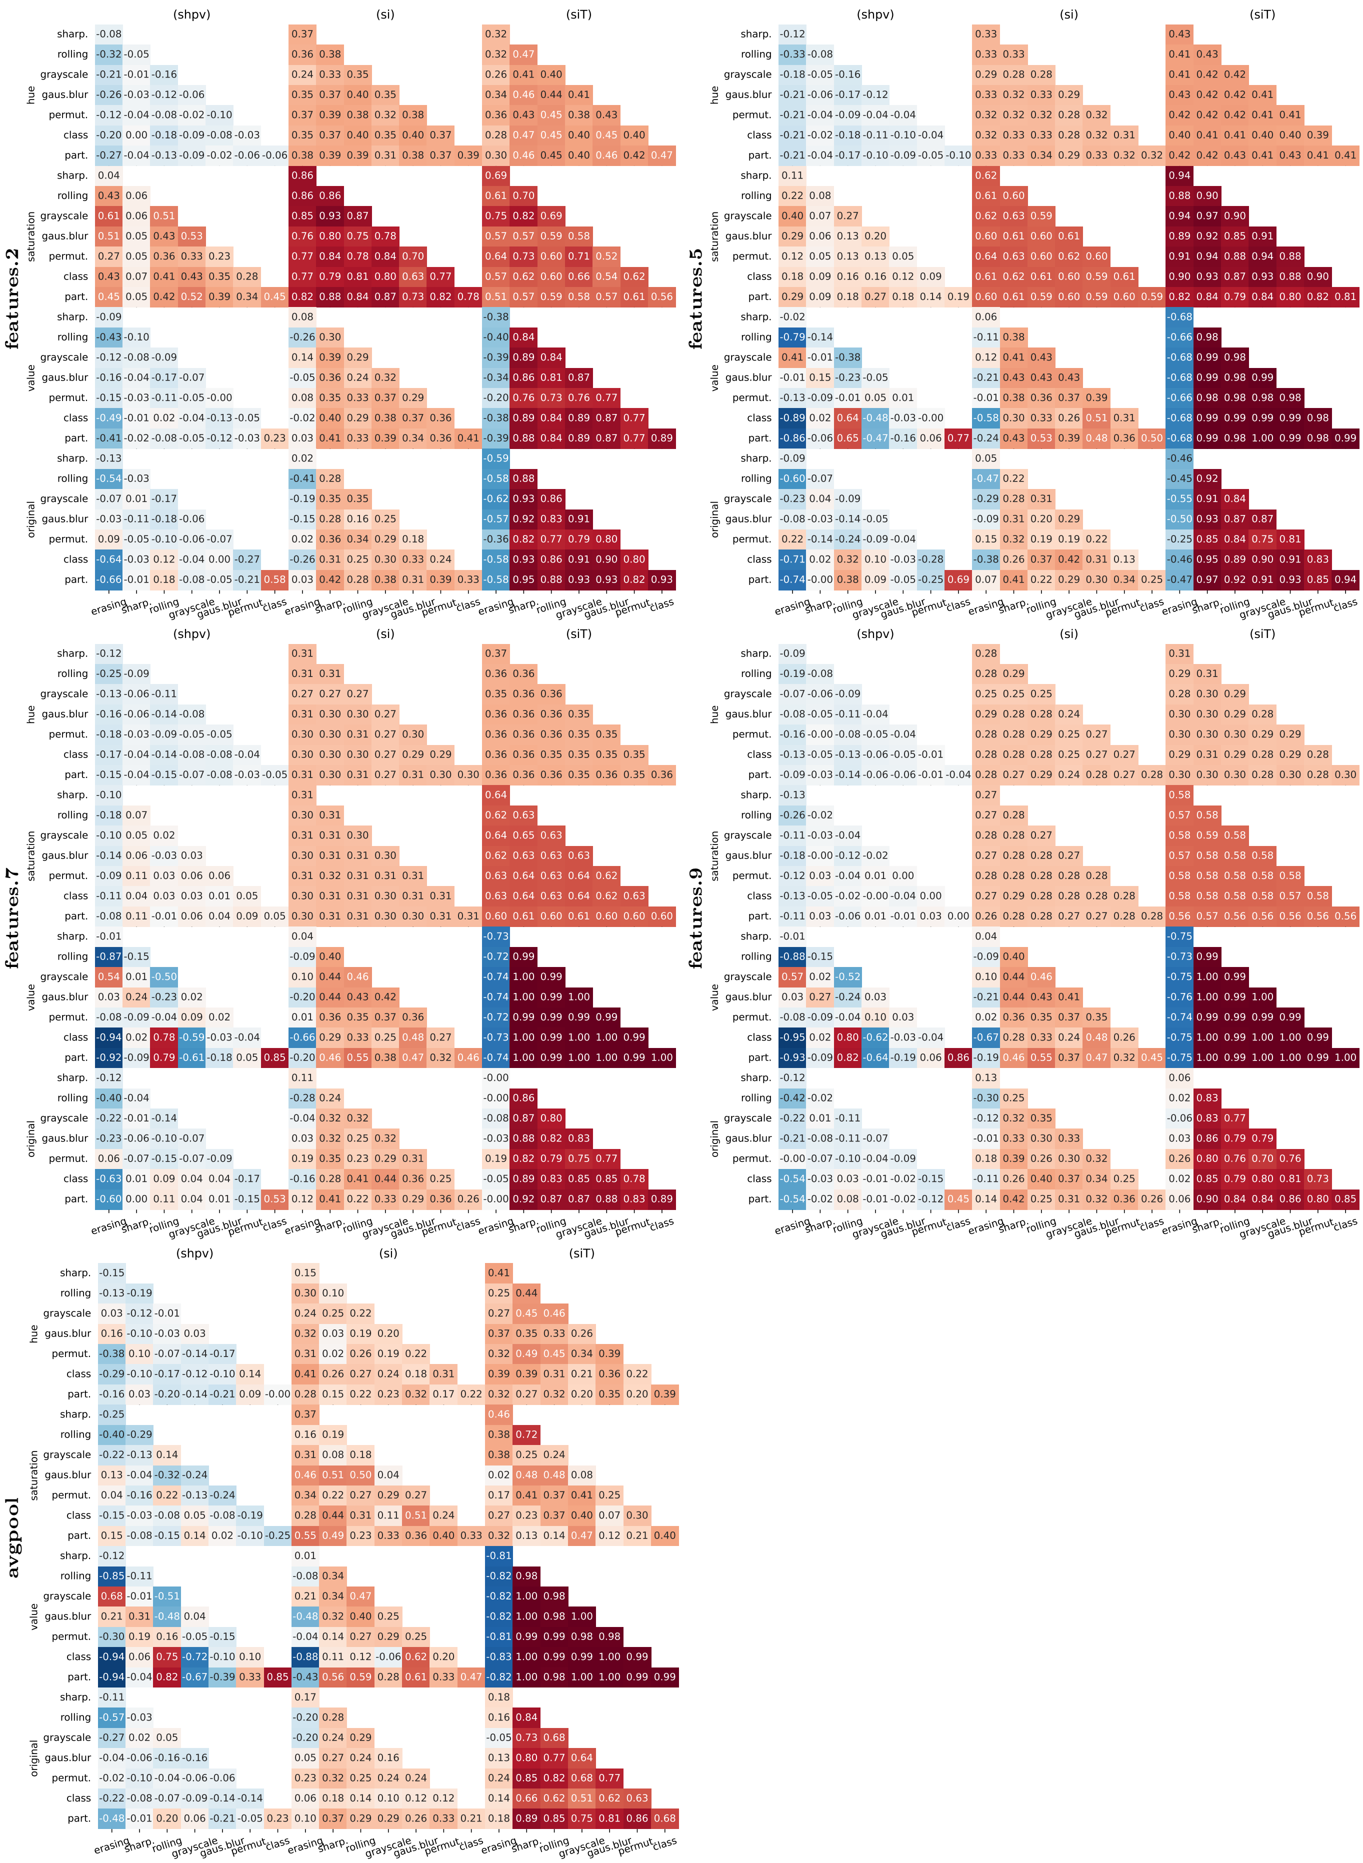


Figure S7.7 (c): Correlation matrices between sensitivity variables for AlexNet (augmentation set 1).

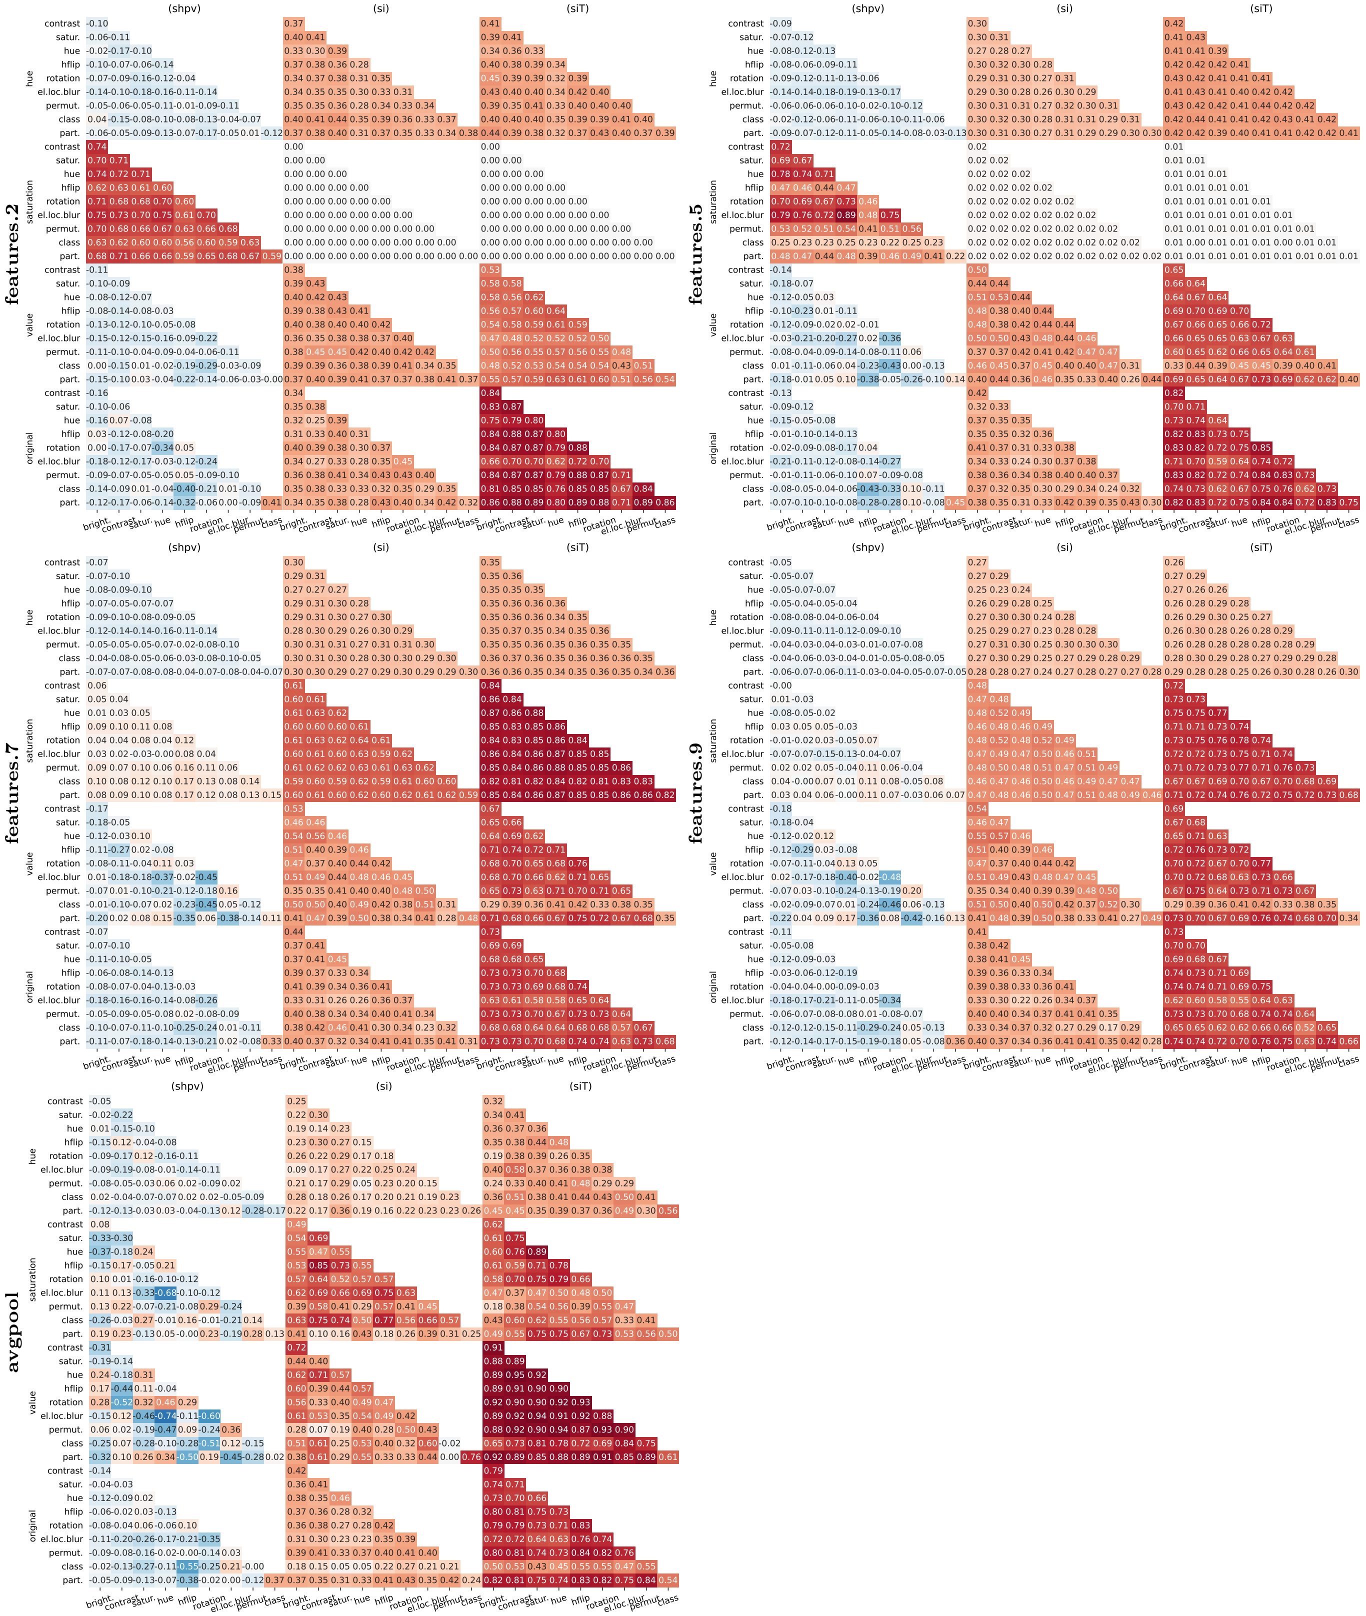


Figure S7.7 (d): Correlation matrices between sensitivity variables for AlexNet (augmentation set 2).
